# Supplementary material for: Visualization for Trust in Machine Learning Revisited: The State of the Field in 2023
Source: arXiv:2403.12005 source file (2024-04-18)
Supplement: Supplementary file 1 [file category_combination_patterns_updated.pdf]

## Frequent category combination patterns

12 patterns with at least 15 categories and data support of at least 10%

| Category combination | Support | Citation keys |
|---|---|---|
| 2D E.1.1 2D<br>Computed E.2.1 Computed<br>Aggregated Inf. E.3.1 Aggregated Information<br>Select E.5.1 Select<br>Explore E.5.2 Explore / Browse<br>Encode E.5.4 Encode<br>Filter E.5.5 Filter / Query<br>Abstract E.5.6 Abstract / Elaborate<br>Connect E.5.7 Connect<br>Color E.6.1 Color<br>Opacity E.6.2 Opacity<br>Performance G.4.3 Performance<br>Visualization Evaluation G.5.2 Visualization Evaluation<br>Metrics Validation G.5.3 Metrics Validation / Results<br>Practitioners H.2 Practitioners / Domain Experts | 66 (12%) | [Arunkumar2023LINGO], [Bauerle2022Symphony], [Boggust2022Embedding], [Caballero2019V], [Cashman2021CAVA], [Cavallo2019Clustrophile2], [Chatzimparmpas2020t-viSNE], [Chatzimparmpas2021StackGenVis], [Chatzimparmpas2021VisEvol], [Chatzimparmpas2022FeatureEnVi], [Chatzimparmpas2023VisRuler], [Chen2016DropoutSeer], [Chen2023Federated], [Cheng2022ACMViz], [Chu2023A], [Das2020QUESTO], [Deng2023Visual], [Feng2023XNLI], [Frohler2016GEMSe], [Ghai2023D], [Guo2021Interpretable], [Hao2023TimeTuner], [Hazarika2019NNVA], [He2022Where], [He2023VideoPro], [Hoque2021Outcome], [Jin2022GNNLens], [Jin2023A], [Kahng2018ActiVis], [Knittel2021Visual], [Kwon2018Clustervision], [Kwon2019RetainVis], [Li2018EmbeddingVis], [Li2023VisualNeuron], [Lin2018RCLens], [Liu2019NLIZE], [Ma2021A], [Ma2021Visual], [Ming2019RuleMatrix], [Munz2022Visualization], [Murugesan2019DeepCompare], [Park2021VATUN], [Pezzotti2018DeepEyes], [Puhringer2020InstanceFlow], [Shao2023Visual], [Sielaff2022Visual], [Sivaraman2022Emblaze], [Spinner2020explAIner], [Teng2023VISPUR], [Tyagi2023NAS], [Wang2019ATMSeer], [Wang2019DQNViz], [Wang2019DeepVID], [Wang2020ConceptExplorer], [Wang2021Visual], [Wang2022M2Lens], [Wang2023CommonsenseVIS], [Wang2023Extending], [Xie2023Towards], [Xu2019EnsembleLens], [Xu2021mTSeer], [Xuan2022VAC], [Zhang2023CohortVA], [Zhang2023LabelVizier], [Zhao2019Oui], [Zhao2019iForest] |
| 2D E.1.1 2D<br>Computed E.2.1 Computed<br>Aggregated Inf. E.3.1 Aggregated Information<br>Instance-based E.3.2 Instance-based / Individual<br>Select E.5.1 Select<br>Explore E.5.2 Explore / Browse<br>Encode E.5.4 Encode<br>Filter E.5.5 Filter / Query<br>Abstract E.5.6 Abstract / Elaborate<br>Connect E.5.7 Connect<br>Color E.6.1 Color<br>Opacity E.6.2 Opacity<br>Performance G.4.3 Performance<br>Visualization Evaluation G.5.2 Visualization Evaluation<br>Metrics Validation G.5.3 Metrics Validation / Results | 64 (11%) | [Alsallakh2018Do], [Arunkumar2023LINGO], [Bauerle2022Symphony], [Boggust2022Embedding], [Cashman2019Ablate], [Cashman2021CAVA], [Cavallo2019Clustrophile2], [Chatzimparmpas2020t-viSNE], [Chatzimparmpas2021StackGenVis], [Chatzimparmpas2021VisEvol], [Chatzimparmpas2022FeatureEnVi], [Chatzimparmpas2023VisRuler], [Chen2016DropoutSeer], [Cheng2022ACMViz], [Das2020QUESTO], [Deng2023Visual], [Dilawer2023MultiCaM], [Feng2023XNLI], [Frohler2016GEMSe], [Guo2021Interpretable], [Hao2023TimeTuner], [Hazarika2019NNVA], [He2022Where], [He2023VideoPro], [Huang2021A], [Jin2023A], [Jin2023ShortcutLens], [Kahng2018ActiVis], [Krause2021Visual], [Kwon2018Clustervision], [Kwon2019RetainVis], [Li2023VisualNeuron], [Lin2018RCLens], [Liu2019NLIZE], [Ma2019Explaining], [Ma2021A], [Ma2021Visual], [Metz2023VISITOR], [Ming2019RuleMatrix], [Munz2022Visualization], [Murugesan2019DeepCompare], [Park2021VATUN], [Pezzotti2018DeepEyes], [Prasad2023ProactiV], [Puhringer2020InstanceFlow], [Shao2023Visual], [Sielaff2022Visual], [Spinner2020explAIner], [Wang2018GANViz], [Wang2019ATMSeer], [Wang2019DQNViz], [Wang2019DeepVID], [Wang2020SCANViz], [Wang2022M2Lens], [Wang2023CommonsenseVIS], [Wang2023Extending], [Wu2023ATICVis], [Xie2023Towards], [Xu2019EnsembleLens], [Xuan2022VAC], [Zhang2023CohortVA], [Zhang2023LabelVizier], [Zhao2019Oui], [Zhao2019iForest] |
| 2D E.1.1 2D<br>Computed E.2.1 Computed<br>Aggregated Inf. E.3.1 Aggregated Information<br>Instance-based E.3.2 Instance-based / Individual<br>Select E.5.1 Select<br>Explore E.5.2 Explore / Browse<br>Encode E.5.4 Encode<br>Filter E.5.5 Filter / Query<br>Abstract E.5.6 Abstract / Elaborate<br>Connect E.5.7 Connect<br>Color E.6.1 Color<br>Performance G.4.3 Performance<br>Visualization Evaluation G.5.2 Visualization Evaluation<br>Metrics Validation G.5.3 Metrics Validation / Results<br>[illegible] | 62 (11%) | [Ahn2019FairSight], [Arunkumar2023LINGO], [Bauerle2022Symphony], [Boggust2022Embedding], [Brooks2015FeatureInsight], [Cashman2019AUser], [Cashman2021CAVA], [Cavallo2019Clustrophile2], [Chatzimparmpas2020t-viSNE], [Chatzimparmpas2021StackGenVis], [Chatzimparmpas2021VisEvol], [Chatzimparmpas2022FeatureEnVi], [Chatzimparmpas2023VisRuler], [Chen2016DropoutSeer], [Chen2018AnchorViz], [Cheng2022ACMViz], [Das2020QUESTO], [Deng2023Visual], [Feng2023XNLI], [Frohler2016GEMSe], [Guo2021Interpretable], [Hao2023TimeTuner], [Hazarika2019NNVA], [He2022Where], [He2023VideoPro], [Jin2023A], [Kahng2018ActiVis], [Krause2017AWorkflow], [Kwon2018Clustervision], [Kwon2019RetainVis], [Li2023VisualNeuron], [Li2023Visual], [Lin2018RCLens], [Liu2019NLIZE], [Ma2021A], [Ma2021Visual], [Ming2019ProtoSteer], [Ming2019RuleMatrix], [Munz2022Visualization], [Murugesan2019DeepCompare], [Park2021VATUN], [Pezzotti2018DeepEyes], [Puhringer2020InstanceFlow], [Shao2023Visual], [Sielaff2022Visual], [Spinner2020explAIner], [Wang2019ATMSeer], [Wang2019DQNViz], [Wang2019DeepVID], |

| | | |
|---|---|---|
| Practitioners H.2 Practitioners / Domain Experts | | [Wang2022M2Lens], [Wang2023CommonsenseVIS], [Wang2023DRAVA], [Wang2023Extending], [Xie2023Towards], [Xu2019EnsembleLens], [Xuan2022VAC], [Yuan2022iSEA], [Zhang2023CohortVA], [Zhang2023LabelVizier], [Zhang2023SliceTeller], [Zhao2019Oui], [Zhao2019iForest] |
| 2D E.1.1 2D<br>Computed E.2.1 Computed<br>Aggregated Inf. E.3.1 Aggregated Information<br>Instance-based E.3.2 Instance-based / Individual<br>Select E.5.1 Select<br>Explore E.5.2 Explore / Browse<br>Encode E.5.4 Encode<br>Filter E.5.5 Filter / Query<br>Abstract E.5.6 Abstract / Elaborate<br>Connect E.5.7 Connect<br>Color E.6.1 Color<br>Opacity E.6.2 Opacity<br>Performance G.4.3 Performance<br>Metrics Validation G.5.3 Metrics Validation / Results<br>Practitioners H.2 Practitioners / Domain Experts | 61<br>(11%) | [Arunkumar2023LINGO], [Bauerle2022Symphony], [Bernard2021ProSeCo], [Boggust2022Embedding], [Cashman2021CAVA], [Cavallo2019Clustrophile2], [Chatzimparmpas2020t-viSNE], [Chatzimparmpas2021StackGenVis], [Chatzimparmpas2021VisEvol], [Chatzimparmpas2022FeatureEnVi], [Chatzimparmpas2023VisRuler], [Chen2016DropoutSeer], [Cheng2022ACMViz], [Das2020QUESTO], [Deng2023Visual], [Feng2023XNLI], [Frohler2016GEMSe], [Gleicher2020Boxer], [Guo2021Interpretable], [Hao2023TimeTuner], [Hazarika2019NNVA], [He2022Where], [He2023VideoPro], [Jin2023A], [Kahng2018ActiVis], [Kwon2018Clustervision], [Kwon2019RetainVis], [Li2023VisualNeuron], [Lin2018RCLens], [Liu2019NLIZE], [Ma2017EasySVM], [Ma2021A], [Ma2021Visual], [Ming2019RuleMatrix], [Munz2022Visualization], [Murugesan2019DeepCompare], [Park2021VATUN], [Pezzotti2018DeepEyes], [Puhringer2020InstanceFlow], [Rostamzadeh2021VERONICA], [Shao2023Visual], [Sielaff2022Visual], [Spinner2020explAIner], [Tamagnini2017Interpreting], [Tenney2020The], [Wang2019ATMSeer], [Wang2019DQNViz], [Wang2019DeepVID], [Wang2021Investigating], [Wang2022M2Lens], [Wang2023CommonsenseVIS], [Wang2023Extending], [Xie2023Towards], [Xu2019EnsembleLens], [Xuan2022VAC], [Zhang2022HyIDSVis], [Zhang2023CohortVA], [Zhang2023LabelVizier], [Zhao2019Oui], [Zhao2019iForest], [Zhao2022Human] |
| 2D E.1.1 2D<br>Computed E.2.1 Computed<br>Mapped E.2.2 Mapped<br>Aggregated Inf. E.3.1 Aggregated Information<br>Instance-based E.3.2 Instance-based / Individual<br>Select E.5.1 Select<br>Explore E.5.2 Explore / Browse<br>Encode E.5.4 Encode<br>Filter E.5.5 Filter / Query<br>Abstract E.5.6 Abstract / Elaborate<br>Connect E.5.7 Connect<br>Color E.6.1 Color<br>Performance G.4.3 Performance<br>Visualization Evaluation G.5.2 Visualization Evaluation<br>Metrics Validation G.5.3 Metrics Validation / Results | 58<br>(10%) | [Ahn2019FairSight], [Alsallakh2018Do], [Arunkumar2023LINGO], [Bauerle2022Symphony], [Boggust2022Embedding], [Brooks2015FeatureInsight], [Cabrera2023Zeno], [Cashman2019AUser], [Cashman2019Ablate], [Cashman2021CAVA], [Cavallo2019Clustrophile2], [Chatzimparmpas2020t-viSNE], [Chatzimparmpas2021StackGenVis], [Chen2016DropoutSeer], [Chen2018AnchorViz], [Chotisarn2021Deep], [Das2020QUESTO], [Dilawer2023MultiCaM], [Feng2023XNLI], [Guo2021Interpretable], [He2022Where], [He2023VideoPro], [Huang2021A], [Kahng2018ActiVis], [Krause2017AWorkflow], [Krause2021Visual], [Kwon2018Clustervision], [Li2021T3], [Li2023VisualNeuron], [Lin2018RCLens], [Liu2019NLIZE], [Ma2019Explaining], [Metz2023VISITOR], [Ming2019ProtoSteer], [Ming2019RuleMatrix], [Munz2022Visualization], [Murugesan2019DeepCompare], [Nie2018Visualizing], [Park2021VATUN], [Pezzotti2018DeepEyes], [Pomme2023NetPrune], [Prasad2023ProactiV], [Puhringer2020InstanceFlow], [Shao2023Visual], [Spinner2020explAIner], [Wang2018GANViz], [Wang2019DQNViz], [Wang2019DeepVID], [Wang2022M2Lens], [Wang2023CommonsenseVIS], [Wu2023ATICVis], [Xu2019EnsembleLens], [Xuan2022VAC], [Yuan2022iSEA], [Zhang2023LabelVizier], [Zhang2023SliceTeller], [Zhao2019Oui], [Zhao2019iForest] |
| 2D E.1.1 2D<br>Computed E.2.1 Computed<br>Aggregated Inf. E.3.1 Aggregated Information<br>Instance-based E.3.2 Instance-based / Individual<br>Select E.5.1 Select<br>Explore E.5.2 Explore / Browse<br>Encode E.5.4 Encode<br>Filter E.5.5 Filter / Query<br>Abstract E.5.6 Abstract / Elaborate<br>Connect E.5.7 Connect<br>Color E.6.1 Color<br>Opacity E.6.2 Opacity<br>Visualization Evaluation G.5.2 Visualization Evaluation<br>Metrics Validation G.5.3 Metrics Validation / Results<br>Practitioners H.2 Practitioners / Domain Experts | 58<br>(10%) | [Arunkumar2023LINGO], [Bauerle2022Symphony], [Boggust2022Embedding], [Cashman2021CAVA], [Cavallo2019Clustrophile2], [Chatzimparmpas2020t-viSNE], [Chatzimparmpas2021StackGenVis], [Chatzimparmpas2021VisEvol], [Chatzimparmpas2022FeatureEnVi], [Chatzimparmpas2023VisRuler], [Chen2016DropoutSeer], [Cheng2022ACMViz], [Collaris2022StrategyAtlas], [Das2020QUESTO], [Deng2023Visual], [Feng2023XNLI], [Floricel2023Roses], [Frohler2016GEMSe], [Guo2021Interpretable], [Hao2023TimeTuner], [Hazarika2019NNVA], [He2022Where], [He2023VideoPro], [Hoque2023Visual], [Jin2023A], [Kahng2018ActiVis], [Kwon2018Clustervision], [Kwon2019RetainVis], [Li2023VisualNeuron], [Lin2018RCLens], [Liu2019NLIZE], [Ma2021A], [Ma2021Visual], [Ming2019RuleMatrix], [Munz2022Visualization], [Murugesan2019DeepCompare], [Park2021VATUN], [Pezzotti2018DeepEyes], [Piringer2010HyperMoVal], [Puhringer2020InstanceFlow], [Shao2023Visual], [Sielaff2022Visual], [Spinner2020explAIner], [Strobelt2019Seq2seq], [Wang2019ATMSeer], [Wang2019DQNViz], [Wang2019DeepVID], [Wang2022M2Lens], [Wang2023CommonsenseVIS], [Wang2023Extending], [Xie2023Towards], [Xu2019EnsembleLens], [Xuan2022VAC], [Zhang2021A], |

| | | |
|---|---|---|
| | | [Zhang2023CohortVA], [Zhang2023LabelVizier], [Zhao2019Oui], [Zhao2019iForest] |
| Classification (sup.) B.2.1.1 Classification<br>2D E.1.1 2D<br>Computed E.2.1 Computed<br>Aggregated Inf. E.3.1 Aggregated Information<br>Instance-based E.3.2 Instance-based / Individual<br>Select E.5.1 Select<br>Explore E.5.2 Explore / Browse<br>Encode E.5.4 Encode<br>Filter E.5.5 Filter / Query<br>Abstract E.5.6 Abstract / Elaborate<br>Connect E.5.7 Connect<br>Color E.6.1 Color<br>Performance G.4.3 Performance<br>Visualization Evaluation G.5.2 Visualization Evaluation<br>Metrics Validation G.5.3 Metrics Validation / Results | 57<br>(10%) | [Ahn2019FairSight], [Alsallakh2018Do], [Bauerle2022Symphony], [Boggust2022Embedding], [Brooks2015FeatureInsight], [Cabrera2023Zeno], [Cashman2019AUser], [Cashman2019Ablate], [Chatzimparmpas2021StackGenVis], [Chatzimparmpas2021VisEvol], [Chatzimparmpas2022FeatureEnVi], [Chatzimparmpas2023VisRuler], [Chen2016DropoutSeer], [Chen2023A], [Das2020QUESTO], [Deng2023Visual], [Dilawer2023MultiCaM], [Guo2021Interpretable], [Hazarika2019NNVA], [Huang2021A], [Jin2023ShortcutLens], [Kahng2018ActiVis], [Krause2017AWorkflow], [Krause2021Visual], [Kwon2019RetainVis], [Li2023VisualNeuron], [Li2023Visual], [Lin2018RCLens], [Liu2019NLIZE], [Ma2019Explaining], [Ma2021A], [Ma2021Visual], [Ming2019ProtoSteer], [Ming2019RuleMatrix], [Murugesan2019DeepCompare], [Nie2018Visualizing], [Park2021VATUN], [Pezzotti2018DeepEyes], [Pomme2023NetPrune], [Prasad2023ProactiV], [Puhringer2020InstanceFlow], [Shao2023Visual], [Sielaff2022Visual], [Spinner2020explAIner], [Wang2018GANViz], [Wang2019ATMSeer], [Wang2020SCANViz], [Wang2022M2Lens], [Wang2023CommonsenseVIS], [Wang2023DRAVA], [Wang2023Extending], [Wu2023ATICVis], [Xie2023Towards], [Xu2019EnsembleLens], [Xuan2022VAC], [Zhang2023SliceTeller], [Zhao2019iForest] |
| Model-agnostic D.1 Model-agnostic / Black Box<br>2D E.1.1 2D<br>Computed E.2.1 Computed<br>Aggregated Inf. E.3.1 Aggregated Information<br>Select E.5.1 Select<br>Explore E.5.2 Explore / Browse<br>Encode E.5.4 Encode<br>Filter E.5.5 Filter / Query<br>Abstract E.5.6 Abstract / Elaborate<br>Connect E.5.7 Connect<br>Color E.6.1 Color<br>Performance G.4.3 Performance<br>Visualization Evaluation G.5.2 Visualization Evaluation<br>Metrics Validation G.5.3 Metrics Validation / Results<br>Practitioners H.2 Practitioners / Domain Experts | 57<br>(10%) | [Ahn2019FairSight], [Arunkumar2023LINGO], [Bauerle2022Symphony], [Boggust2022Embedding], [Brooks2015FeatureInsight], [Caballero2019V], [Cashman2019AUser], [Cashman2021CAVA], [Cavallo2019Clustrophile2], [Chatzimparmpas2021StackGenVis], [Chatzimparmpas2021VisEvol], [Chatzimparmpas2022FeatureEnVi], [Chen2016DropoutSeer], [Chen2018AnchorViz], [Chen2023Federated], [Chu2023A], [Das2020QUESTO], [Feng2023XNLI], [Frohler2016GEMSe], [Ghai2023D], [Guo2021Interpretable], [Hao2023TimeTuner], [Hazarika2019NNVA], [He2022Where], [He2023VideoPro], [Hoque2021Outcome], [Jin2022GNNLens], [Krause2017AWorkflow], [Kwon2018Clustervision], [Li2018EmbeddingVis], [Lin2018RCLens], [Liu2019NLIZE], [Ma2021A], [Ma2021Visual], [Ming2019RuleMatrix], [Murugesan2019DeepCompare], [Pezzotti2018DeepEyes], [Sivaraman2022Emblaze], [Spinner2020explAIner], [Teng2023VISPUR], [Wang2019ATMSeer], [Wang2019DeepVID], [Wang2020ConceptExplorer], [Wang2021Visual], [Wang2022M2Lens], [Wang2023CommonsenseVIS], [Wang2023DRAVA], [Xie2023Towards], [Xu2019EnsembleLens], [Xu2021mTSeer], [Yuan2022VisualExploration], [Yuan2022iSEA], [Zhang2023CohortVA], [Zhang2023LabelVizier], [Zhang2023SliceTeller], [Zhao2019Oui] |
| 2D E.1.1 2D<br>Computed E.2.1 Computed<br>Aggregated Inf. E.3.1 Aggregated Information<br>Instance-based E.3.2 Instance-based / Individual<br>Select E.5.1 Select<br>Explore E.5.2 Explore / Browse<br>Filter E.5.5 Filter / Query<br>Abstract E.5.6 Abstract / Elaborate<br>Connect E.5.7 Connect<br>Color E.6.1 Color<br>Opacity E.6.2 Opacity<br>Performance G.4.3 Performance<br>Visualization Evaluation G.5.2 Visualization Evaluation<br>Metrics Validation G.5.3 Metrics Validation / Results<br>Practitioners H.2 Practitioners / Domain Experts | 57<br>(10%) | [Antweiler2022Visualizing], [Arunkumar2023LINGO], [Bauerle2022Symphony], [Boggust2022Embedding], [Cashman2021CAVA], [Cavallo2019Clustrophile2], [Chatzimparmpas2020t-viSNE], [Chatzimparmpas2021StackGenVis], [Chatzimparmpas2021VisEvol], [Chatzimparmpas2022FeatureEnVi], [Chatzimparmpas2023HardVis], [Chatzimparmpas2023VisRuler], [Chen2016DropoutSeer], [Cheng2022ACMViz], [Das2020QUESTO], [Deng2023Visual], [Feng2023XNLI], [Frohler2016GEMSe], [Guo2021Interpretable], [Hao2023TimeTuner], [Hazarika2019NNVA], [He2022Where], [He2023VideoPro], [Jin2023A], [Kahng2018ActiVis], [Kwon2018Clustervision], [Kwon2019RetainVis], [Li2022A], [Li2023VisualNeuron], [Lin2018RCLens], [Liu2019NLIZE], [Ma2021A], [Ma2021Visual], [Ming2019RuleMatrix], [Munz2022Visualization], [Murugesan2019DeepCompare], [Park2021VATUN], [Pezzotti2018DeepEyes], [Puhringer2020InstanceFlow], [Shao2023Visual], [Sielaff2022Visual], [Spinner2020explAIner], [Suschnigg2021Visual], [Wang2019ATMSeer], [Wang2019DQNViz], [Wang2019DeepVID], [Wang2022M2Lens], [Wang2022When], [Wang2023CommonsenseVIS], [Wang2023Extending], [Xie2023Towards], [Xu2019EnsembleLens], [Xuan2022VAC], [Zhang2023CohortVA], [Zhang2023LabelVizier], [Zhao2019Oui], [Zhao2019iForest] |
| 2D E.1.1 2D<br>Computed E.2.1 Computed<br>Aggregated Inf. E.3.1 Aggregated Information<br>Bar Charts E.4.1 Bar Charts | 56<br>(10%) | [Ahn2019FairSight], [Bauerle2022Symphony], [Boggust2022Embedding], [Brooks2015FeatureInsight], [Caballero2019V], [Cashman2019AUser], [Cavallo2019Clustrophile2], [Chatzimparmpas2020t-viSNE], [Chatzimparmpas2021StackGenVis], [Chatzimparmpas2021VisEvol], [Chatzimparmpas2022FeatureEnVi], [Chatzimparmpas2023VisRuler], |

| | | |
|---|---|---|
| Select E.5.1 Select<br>Explore E.5.2 Explore / Browse<br>Encode E.5.4 Encode<br>Filter E.5.5 Filter / Query<br>Abstract E.5.6 Abstract / Elaborate<br>Connect E.5.7 Connect<br>Color E.6.1 Color<br>Performance G.4.3 Performance<br>Visualization Evaluation G.5.2 Visualization Evaluation<br>Metrics Validation G.5.3 Metrics Validation / Results<br>Practitioners H.2 Practitioners / Domain Experts | | [Chen2016DropoutSeer], [Cheng2022ACMViz], [Chu2023A], [Deng2023Visual], [Feng2023XNLI], [Ghai2023D], [Hao2023TimeTuner], [Hazarika2019NNVA], [He2023VideoPro], [Hoque2021Outcome], [Jin2022GNNLens], [Knittel2021Visual], [Krause2017AWorkflow], [Kwon2018Clustervision], [Kwon2019RetainVis], [Li2018EmbeddingVis], [Lin2018RCLens], [Ma2021Visual], [Ming2019ProtoSteer], [Ming2019RuleMatrix], [Munz2022Visualization], [Puhringer2020InstanceFlow], [Shao2023Visual], [Sielaff2022Visual], [Sivaraman2022Emblaze], [Teng2023VISPUR], [Wang2019ATMSeer], [Wang2019DQNViz], [Wang2019DeepVID], [Wang2021Visual], [Wang2023DRAVA], [Xu2019EnsembleLens], [Xu2021mTSeer], [Xuan2022VAC], [Yuan2022VisualExploration], [Yuan2022iSEA], [Zhang2023CohortVA], [Zhang2023LabelVizier], [Zhang2023SliceTeller], [Zhao2019Oui], [Zhao2019iForest] |
| Model-agnostic D.1 Model-agnostic / Black Box<br>2D E.1.1 2D<br>Computed E.2.1 Computed<br>Aggregated Inf. E.3.1 Aggregated Information<br>Select E.5.1 Select<br>Explore E.5.2 Explore / Browse<br>Encode E.5.4 Encode<br>Filter E.5.5 Filter / Query<br>Abstract E.5.6 Abstract / Elaborate<br>Connect E.5.7 Connect<br>Color E.6.1 Color<br>Opacity E.6.2 Opacity<br>Performance G.4.3 Performance<br>Visualization Evaluation G.5.2 Visualization Evaluation<br>Metrics Validation G.5.3 Metrics Validation / Results | 55 (10%) | [Alsallakh2018Do], [Arunkumar2023LINGO], [Bauerle2022Symphony], [Boggust2022Embedding], [Caballero2019V], [Cashman2019Ablate], [Cashman2021CAVA], [Cavallo2019Clustrophile2], [Chatzimparmpas2021StackGenVis], [Chatzimparmpas2021VisEvol], [Chatzimparmpas2022FeatureEnVi], [Chen2016DropoutSeer], [Chen2023Federated], [Chu2023A], [Das2020QUESTO], [Dilawer2023MultiCaM], [Feng2023XNLI], [Frohler2016GEMSe], [Ghai2023D], [Guo2021Interpretable], [Hao2023TimeTuner], [Hazarika2019NNVA], [He2022Where], [He2023VideoPro], [Hoque2021Outcome], [Jin2022GNNLens], [Jin2023ShortcutLens], [Krause2021Visual], [Kwon2018Clustervision], [Li2018EmbeddingVis], [Lin2018RCLens], [Liu2019NLIZE], [Ma2019Explaining], [Ma2021A], [Ma2021Visual], [Ming2019RuleMatrix], [Murugesan2019DeepCompare], [Pezzotti2018DeepEyes], [Prasad2023ProactiV], [Sivaraman2022Emblaze], [Spinner2020explAIner], [Talbot2009EnsembleMatrix], [Teng2023VISPUR], [Wang2019ATMSeer], [Wang2019DeepVID], [Wang2020ConceptExplorer], [Wang2021Visual], [Wang2022M2Lens], [Wang2023CommonsenseVIS], [Xie2023Towards], [Xu2019EnsembleLens], [Xu2021mTSeer], [Zhang2023CohortVA], [Zhang2023LabelVizier], [Zhao2019Oui] |
| 2D E.1.1 2D<br>Computed E.2.1 Computed<br>Aggregated Inf. E.3.1 Aggregated Information<br>Instance-based E.3.2 Instance-based / Individual<br>Select E.5.1 Select<br>Explore E.5.2 Explore / Browse<br>Encode E.5.4 Encode<br>Abstract E.5.6 Abstract / Elaborate<br>Connect E.5.7 Connect<br>Color E.6.1 Color<br>Opacity E.6.2 Opacity<br>Performance G.4.3 Performance<br>Visualization Evaluation G.5.2 Visualization Evaluation<br>Metrics Validation G.5.3 Metrics Validation / Results<br>Practitioners H.2 Practitioners / Domain Experts | 55 (10%) | [Arunkumar2023LINGO], [Bauerle2022Symphony], [Boggust2022Embedding], [Cashman2021CAVA], [Cavallo2019Clustrophile2], [Chatzimparmpas2020t-viSNE], [Chatzimparmpas2021StackGenVis], [Chatzimparmpas2021VisEvol], [Chatzimparmpas2022FeatureEnVi], [Chatzimparmpas2023VisRuler], [Chen2016DropoutSeer], [Cheng2022ACMViz], [Collaris2020ExplainExplore], [Das2020QUESTO], [Deng2023Visual], [Feng2023XNLI], [Frohler2016GEMSe], [Guo2021Interpretable], [Hao2023TimeTuner], [Hazarika2019NNVA], [He2022Where], [He2023VideoPro], [Jin2023A], [Kahng2018ActiVis], [Kwon2018Clustervision], [Kwon2019RetainVis], [Kwon2022RMExplorer], [Li2023VisualNeuron], [Lin2018RCLens], [Liu2019NLIZE], [Ma2021A], [Ma2021Visual], [Ming2019RuleMatrix], [Munz2022Visualization], [Murugesan2019DeepCompare], [Park2021VATUN], [Pezzotti2018DeepEyes], [Puhringer2020InstanceFlow], [Shao2023Visual], [Sielaff2022Visual], [Spinner2020explAIner], [Velumani2022AQX], [Wang2019ATMSeer], [Wang2019DQNViz], [Wang2019DeepVID], [Wang2022M2Lens], [Wang2023CommonsenseVIS], [Wang2023Extending], [Xie2023Towards], [Xu2019EnsembleLens], [Xuan2022VAC], [Zhang2023CohortVA], [Zhang2023LabelVizier], [Zhao2019Oui], [Zhao2019iForest] |
