# Supplementary material for: Visualization for Trust in Machine Learning Revisited: The State of the Field in 2023
Source: arXiv:2403.12005 source file (2024-04-18)
Supplement: Supplementary file 2 [file S7.tex]

\documentclass[a4paper]{article}

\usepackage[a4paper,margin=1cm]{geometry}

\usepackage{hyperref}

\usepackage{graphicx}
\usepackage[dvipsnames]{xcolor}

\usepackage{rotating}
\usepackage{multirow}
\usepackage{pbox}

\usepackage{xstring}

% ---------------------------------------------------------------------

\newcommand{\cit}[1]{``#1''}
\newcommand{\ignore}[1]{}
\newcommand{\todo}[1]{\noindent\fcolorbox[rgb]{0.9,0,0}{1,1,0.8}{\parbox{0.97\columnwidth}{TODO: #1}}\newline}
\newcommand{\filledcell}{\raisebox{-0.3\height}{\color[rgb]{0,0.5,0}{\Large \textbullet}}}
\newcommand{\categoryicon}[1]{\raisebox{-0.2\height}{\includegraphics[height=\baselineskip]{images/icon-#1.png}}}
\newcommand{\tableicon}[1]{\raisebox{-0.38\height}{\includegraphics[height=2.7mm]{images/icon-#1.png}}}
\newcommand{\tabledescr}[1]{\scalebox{.8}{\begin{sideways}\pbox[c]{\textwidth}{#1}\end{sideways}}}
\newcommand{\tableheader}[2]{\parbox[b]{3mm}{\centering \tabledescr{#1}}}

\newcommand{\headercell}[2]{\parbox[b]{1cm}{\noindent\raisebox{0.5\height}{\fcolorbox[rgb]{0,0,0}{#1}{\scriptsize~}}\,\resizebox{0.62cm}{!}{#2}}}
\newcommand{\colorcell}[2]{\noindent\raisebox{0.5\height}{\fcolorbox[rgb]{0,0,0}{#1}{\scriptsize~}}\,\tiny#2}

%% KK: the original version used the keys from STAR_EuroVis2020.aux 
%% As the current manuscript no longer uses CGF/abbrv Bib keys, relying on internal IDs instead
\newcommand{\inlinecite}[1]{#1}

\hypersetup{
	pdfinfo={
		Title={Visualization for Trust in Machine Learning Revisited: The State of the Field in 2023 - Authorship Statistics},
		Author={A. Chatzimparmpas, K. Kucher, A. Kerren},
		Keywords={trustworthy machine learning; visualization; interpretable machine learning; explainable machine learning},
	}
}

\title{Visualization for Trust in Machine Learning Revisited:\\The State of the Field in 2023 --- Authorship Statistics}
\author{}
\date{}

%-------------------------------------------------------------------------
\begin{document}
\pagenumbering{gobble}
\maketitle
%\vspace{-20mm}

\begin{table}[th!]
	\centering
	\noindent%

	\begin{tabular}{|l|c|c|c|c|c|c|c|c|c|c|c|c|c|c|}
		\hline
		\textbf{\#techniques} & 1 & 2 & 3 & 4 & 5 & 6 & 7 & 8 & 10 \\
		\hline
		\textbf{\#authors} & 453 & 68 & 41 & 23 & 8 & 3 & 2 & 3 & 1 \\
		\hline
		\textbf{\%authors} & 75.2 & 11.3 & 6.8 & 3.8 & 1.3 & 0.5 & 0.3 & 0.5 & 0.2 \\
		\hline
	\end{tabular}%

	\caption{Authorship count distribution for the original 2020 STAR survey data. 
		The respective data set includes \textbf{200} techniques/papers, \textbf{602} unique authors, and \textbf{910} authorship entries in total. 
		Note that 453 out of 602 authors (75.2\%) are only found in a single paper in this data set.}
	\label{tab:author-distribution-2020}
\end{table}

\begin{table}[th!]
	\centering
	\noindent%
	
	\begin{tabular}{|l|c|c|c|c|c|c|c|c|c|c|c|c|c|c|c|c|c|c|}
		\hline
		\textbf{\#techniques} & 1 & 2 & 3 & 4 & 5 & 6 & 7 & 8 & 9 & 10 & 11 & 12 & 13 & 14 & 15 & 16 & 17 & 26 \\
		\hline
		\textbf{\#authors} & 1129 & 204 & 79 & 35 & 33 & 16 & 5 & 12 & 6 & 3 & 3 & 1 & 2 & 4 & 2 & 2 & 2 & 1  \\
		\hline
		\textbf{\%authors} & 73.4 & 13.3 & 5.1 & 2.3 & 2.1 & 1.0 & 0.3 & 0.8 & 0.4 & 0.2 & 0.2 & 0.1 & 0.1 & 0.3 & 0.1 & 0.1 & 0.1 & 0.1  \\
		\hline
	\end{tabular}%
	
	\caption{Authorship count distribution for the updated 2023 survey data. 
		The respective data set includes \textbf{542} techniques/papers (2.71 times increase from the 2020 data), \textbf{1,539} unique authors (2.56 times increase), and \textbf{2,639} authorship entries in total (2.9 times increase). 
		Note that 1,129 out of 1,539 authors (73.4\%) are only found in a single paper in this data set.
		}
	\label{tab:author-distribution-2023}
\end{table}

\begin{figure}[th!]
	\centering
	\noindent%
	
	\includegraphics[width=\textwidth]{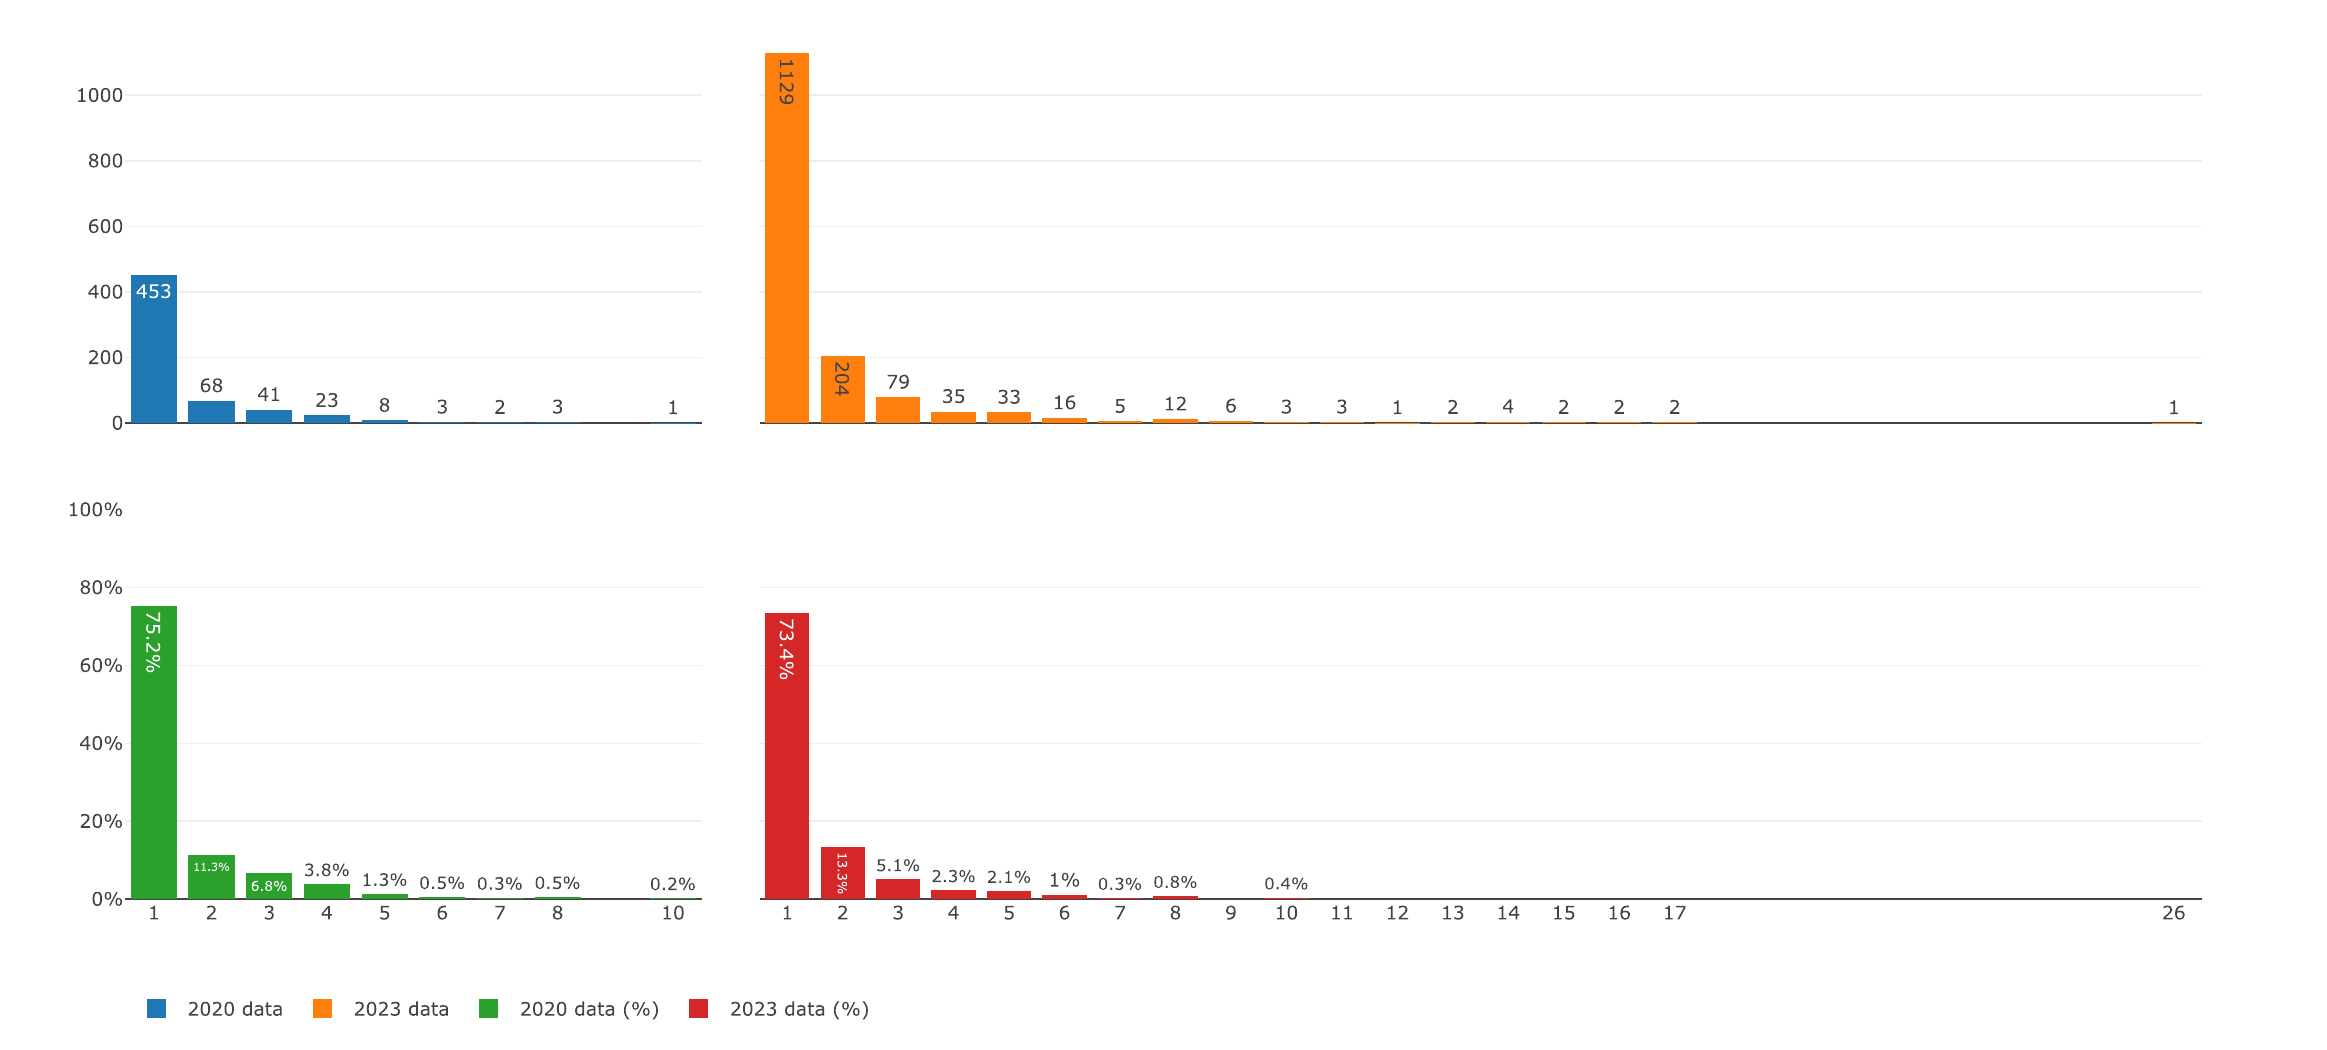}
	
	\caption{Histograms representing the data from the tables above.
	}
	\label{fig:author-distributions}
\end{figure}

\end{document}
