# Supplementary material for: Visualization for Trust in Machine Learning Revisited: The State of the Field in 2023
Source: arXiv:2403.12005 source file (2024-04-18)
Supplement: Supplementary file 3 [file topic_modeling.pdf]

# Visualization for Trust in Machine Learning Revisited: The State of the Field in 2023 — Topic Modeling Results

Table 1: The topic modeling results for our survey (as of September 20, 2023). See the updated survey data at `https://trustmlvis.lnu.se`

| # | Technique | Topic_1 | Topic_2 | Topic_3 | Topic_4 | Topic_5 | Topic_6 | Topic_7 | Topic_8 | Topic_9 | Topic_10 |
|---|---|---|---|---|---|---|---|---|---|---|---|
| 1 | Aupetit2007Visualizing | 0.00 | 0.00 | 0.00 | 0.19 | 0.15 | 0.00 | 0.66 | 0.00 | 0.00 | 0.00 |
| 2 | Garg2008Model | 0.00 | 0.07 | 0.03 | 0.03 | 0.19 | 0.19 | 0.15 | 0.00 | 0.00 | 0.33 |
| 3 | Crossno2009LSAView | 0.00 | 0.11 | 0.00 | 0.05 | 0.00 | 0.65 | 0.00 | 0.00 | 0.18 | 0.00 |
| 4 | Jeong2009iPCA | 0.19 | 0.00 | 0.00 | 0.00 | 0.00 | 0.23 | 0.59 | 0.00 | 0.00 | 0.00 |
| 5 | Johansson2009Interactive | 0.00 | 0.84 | 0.00 | 0.00 | 0.00 | 0.15 | 0.00 | 0.00 | 0.00 | 0.00 |
| 6 | Sips2009Selecting | 0.00 | 0.59 | 0.00 | 0.00 | 0.20 | 0.21 | 0.00 | 0.00 | 0.00 | 0.00 |
| 7 | Talbot2009EnsembleMatrix | 0.03 | 0.00 | 0.00 | 0.00 | 0.26 | 0.25 | 0.00 | 0.06 | 0.00 | 0.40 |
| 8 | VanLong2009MultiClusterTree | 0.00 | 0.38 | 0.00 | 0.16 | 0.00 | 0.46 | 0.00 | 0.00 | 0.00 | 0.00 |
| 9 | Choo2010iVisClassifier | 0.00 | 0.00 | 0.00 | 0.00 | 0.09 | 0.91 | 0.00 | 0.00 | 0.00 | 0.00 |
| 10 | Ingram2010DimStiller | 0.00 | 0.80 | 0.00 | 0.00 | 0.00 | 0.16 | 0.04 | 0.00 | 0.00 | 0.00 |
| 11 | Kapoor2010Interactive | 0.14 | 0.00 | 0.00 | 0.00 | 0.23 | 0.26 | 0.00 | 0.13 | 0.00 | 0.24 |
| 12 | MacInnes2010Visual | 0.00 | 0.00 | 0.00 | 0.00 | 0.00 | 0.34 | 0.00 | 0.11 | 0.00 | 0.56 |
| 13 | Migut2010Visual | 0.10 | 0.25 | 0.00 | 0.00 | 0.52 | 0.00 | 0.00 | 0.00 | 0.00 | 0.12 |
| 14 | Piringer2010HyperMoVal | 0.00 | 0.00 | 0.00 | 0.00 | 0.96 | 0.00 | 0.00 | 0.00 | 0.00 | 0.04 |
| 15 | Schreck2010Techniques | 0.00 | 0.00 | 0.00 | 0.00 | 0.89 | 0.00 | 0.11 | 0.00 | 0.00 | 0.00 |
| 16 | Seifert2010Stress | 0.00 | 0.00 | 0.00 | 0.23 | 0.56 | 0.21 | 0.00 | 0.00 | 0.00 | 0.00 |
| 17 | Ahmed2011Steerable | 0.00 | 0.09 | 0.00 | 0.00 | 0.00 | 0.64 | 0.14 | 0.00 | 0.02 | 0.11 |
| 18 | Albuquerque2011Perception | 0.00 | 0.00 | 0.00 | 0.03 | 0.24 | 0.08 | 0.66 | 0.00 | 0.00 | 0.00 |
| 19 | Berger2011Uncertainty | 0.00 | 0.00 | 0.00 | 0.00 | 0.86 | 0.00 | 0.14 | 0.00 | 0.00 | 0.00 |
| 20 | Bremm2011Assisted | 0.00 | 0.03 | 0.00 | 0.00 | 0.19 | 0.63 | 0.14 | 0.00 | 0.00 | 0.00 |
| 21 | Lespinats2011CheckViz | 0.00 | 0.00 | 0.00 | 0.49 | 0.47 | 0.00 | 0.03 | 0.00 | 0.00 | 0.00 |
| 22 | May2011Guiding | 0.00 | 0.96 | 0.00 | 0.00 | 0.00 | 0.00 | 0.04 | 0.00 | 0.00 | 0.00 |
| 23 | Migut2011Interactive | 0.15 | 0.03 | 0.00 | 0.00 | 0.41 | 0.31 | 0.00 | 0.00 | 0.00 | 0.10 |
| 24 | Turkay2011Interactive | 0.00 | 0.03 | 0.00 | 0.00 | 0.00 | 0.87 | 0.10 | 0.00 | 0.00 | 0.00 |
| 25 | VanDenElzen2011BaobabView | 0.00 | 1.00 | 0.00 | 0.00 | 0.00 | 0.00 | 0.00 | 0.00 | 0.00 | 0.00 |
| 26 | Amorim2012iLAMP | 0.00 | 0.00 | 0.00 | 0.00 | 1.00 | 0.00 | 0.00 | 0.00 | 0.00 | 0.00 |
| 27 | Brown2012Dis | 0.00 | 0.00 | 0.00 | 0.00 | 0.10 | 0.28 | 0.60 | 0.00 | 0.00 | 0.02 |
| 28 | Engel2012Visual | 0.00 | 0.00 | 0.00 | 0.82 | 0.05 | 0.02 | 0.12 | 0.00 | 0.00 | 0.00 |
| 29 | Hoferlin2012Inter | 0.00 | 0.02 | 0.00 | 0.00 | 0.53 | 0.00 | 0.06 | 0.39 | 0.00 | 0.00 |
| 30 | Jankowska2012Relative | 0.00 | 0.00 | 0.00 | 1.00 | 0.00 | 0.00 | 0.00 | 0.00 | 0.00 | 0.00 |
| 31 | Kienreich2012Visual | 0.00 | 0.25 | 0.00 | 0.00 | 0.23 | 0.52 | 0.00 | 0.00 | 0.00 | 0.00 |
| 32 | Lee2012iVisClustering | 0.00 | 0.00 | 0.00 | 0.00 | 0.00 | 1.00 | 0.00 | 0.00 | 0.00 | 0.00 |
| 33 | Paiva2012Semi | 0.00 | 0.28 | 0.00 | 0.00 | 0.31 | 0.37 | 0.03 | 0.00 | 0.00 | 0.00 |
| 34 | Tatu2012Subspace | 0.00 | 0.03 | 0.00 | 0.00 | 0.00 | 0.97 | 0.00 | 0.00 | 0.00 | 0.00 |
| 35 | Fernstad2013Quality | 0.00 | 0.84 | 0.00 | 0.00 | 0.00 | 0.16 | 0.00 | 0.00 | 0.00 | 0.00 |
| 36 | Gleicher2013Explainers | 0.00 | 0.19 | 0.00 | 0.00 | 0.37 | 0.00 | 0.00 | 0.00 | 0.00 | 0.42 |
| 37 | Muhlbacher2013APartition | 0.00 | 0.46 | 0.00 | 0.00 | 0.16 | 0.00 | 0.29 | 0.00 | 0.07 | 0.00 |
| 38 | Alsallakh2014Visual | 0.00 | 0.95 | 0.00 | 0.00 | 0.05 | 0.00 | 0.00 | 0.00 | 0.00 | 0.00 |
| 39 | Bogl2014Visual | 0.00 | 0.29 | 0.00 | 0.00 | 0.00 | 0.00 | 0.04 | 0.00 | 0.52 | 0.15 |
| 40 | Chuang2014Interactive | 0.00 | 0.17 | 0.00 | 0.43 | 0.00 | 0.00 | 0.00 | 0.26 | 0.00 | 0.14 |
| 41 | Gotz2014Visualizing | 0.00 | 0.00 | 0.00 | 0.00 | 0.00 | 0.00 | 0.00 | 0.00 | 0.15 | 0.85 |
| 42 | Krause2014INFUSE | 0.03 | 0.59 | 0.00 | 0.00 | 0.00 | 0.00 | 0.00 | 0.00 | 0.00 | 0.38 |
| 43 | Lee2014A | 0.00 | 0.00 | 0.00 | 0.44 | 0.00 | 0.12 | 0.44 | 0.00 | 0.00 | 0.00 |
| 44 | Liu2014Distortion | 0.00 | 0.00 | 0.00 | 0.69 | 0.12 | 0.16 | 0.03 | 0.00 | 0.00 | 0.00 |
| 45 | Martins2014Visual | 0.00 | 0.00 | 0.00 | 0.00 | 1.00 | 0.00 | 0.00 | 0.00 | 0.00 | 0.00 |
| 46 | Molchanov2014Interactive | 0.00 | 0.07 | 0.00 | 0.00 | 0.58 | 0.23 | 0.13 | 0.00 | 0.00 | 0.00 |
| 47 | Padua2014Interactive | 0.00 | 1.00 | 0.00 | 0.00 | 0.00 | 0.00 | 0.00 | 0.00 | 0.00 | 0.00 |
| 48 | Rieck2014Enhancing | 0.00 | 0.14 | 0.00 | 0.53 | 0.33 | 0.00 | 0.00 | 0.00 | 0.00 | 0.00 |
| 49 | Stolper2014Progressive | 0.00 | 0.06 | 0.10 | 0.00 | 0.00 | 0.00 | 0.38 | 0.00 | 0.14 | 0.32 |
| 50 | Zeiler2014Visualizing | 0.00 | 0.00 | 0.47 | 0.00 | 0.53 | 0.00 | 0.00 | 0.00 | 0.00 | 0.00 |

Table 2: The topic modeling results for our survey (continued).

| # | Technique | Topic_1 | Topic_2 | Topic_3 | Topic_4 | Topic_5 | Topic_6 | Topic_7 | Topic_8 | Topic_9 | Topic_10 |
|---|---|---|---|---|---|---|---|---|---|---|---|
| 51 | Zhao2014LoVis | 0.00 | 0.30 | 0.00 | 0.00 | 0.49 | 0.11 | 0.00 | 0.00 | 0.00 | 0.09 |
| 52 | Amershi2015ModelTracker | 0.00 | 0.00 | 0.00 | 0.00 | 0.07 | 0.04 | 0.00 | 0.08 | 0.00 | 0.81 |
| 53 | Bogl2015Integrating | 0.00 | 0.29 | 0.00 | 0.00 | 0.00 | 0.00 | 0.11 | 0.00 | 0.60 | 0.00 |
| 54 | Brooks2015FeatureInsight | 0.00 | 0.00 | 0.00 | 0.09 | 0.00 | 0.08 | 0.00 | 0.11 | 0.00 | 0.73 |
| 55 | Coimbra2016Explaining | 0.00 | 0.05 | 0.00 | 0.00 | 0.95 | 0.00 | 0.00 | 0.00 | 0.00 | 0.00 |
| 56 | Joia2015Uncovering | 0.00 | 0.09 | 0.00 | 0.00 | 0.10 | 0.81 | 0.00 | 0.00 | 0.00 | 0.00 |
| 57 | Kulesza2015Principles | 0.82 | 0.00 | 0.00 | 0.00 | 0.00 | 0.04 | 0.00 | 0.14 | 0.00 | 0.00 |
| 58 | Liu2015Visual | 0.00 | 0.00 | 0.00 | 0.13 | 0.34 | 0.52 | 0.00 | 0.00 | 0.00 | 0.00 |
| 59 | Rauber2015Interactive | 0.00 | 0.09 | 0.00 | 0.00 | 0.84 | 0.08 | 0.00 | 0.00 | 0.00 | 0.00 |
| 60 | Rieck2015Comparing | 0.00 | 0.00 | 0.00 | 1.00 | 0.00 | 0.00 | 0.00 | 0.00 | 0.00 | 0.00 |
| 61 | Rieck2015Persistent | 0.00 | 0.00 | 0.00 | 1.00 | 0.00 | 0.00 | 0.00 | 0.00 | 0.00 | 0.00 |
| 62 | Silva2015Attribute | 0.03 | 0.05 | 0.00 | 0.05 | 0.66 | 0.21 | 0.00 | 0.00 | 0.00 | 0.00 |
| 63 | Yosinski2015Understanding | 0.00 | 0.00 | 0.25 | 0.00 | 0.75 | 0.00 | 0.00 | 0.00 | 0.00 | 0.00 |
| 64 | Assala2016Interactive | 0.00 | 0.00 | 0.00 | 0.00 | 0.00 | 1.00 | 0.00 | 0.00 | 0.00 | 0.00 |
| 65 | Chen2016DropoutSeer | 0.00 | 0.00 | 0.00 | 0.00 | 0.00 | 0.01 | 0.00 | 0.00 | 0.79 | 0.20 |
| 66 | Frohler2016GEMSe | 0.00 | 0.02 | 0.07 | 0.00 | 0.35 | 0.56 | 0.00 | 0.00 | 0.00 | 0.00 |
| 67 | Gotz2016Adaptive | 0.29 | 0.04 | 0.00 | 0.00 | 0.00 | 0.15 | 0.00 | 0.00 | 0.00 | 0.51 |
| 68 | Kahng2016Visual | 0.00 | 0.15 | 0.00 | 0.00 | 0.00 | 0.00 | 0.00 | 0.11 | 0.00 | 0.75 |
| 69 | Krause2016Interacting | 0.00 | 0.00 | 0.00 | 0.00 | 0.05 | 0.00 | 0.00 | 0.00 | 0.00 | 0.95 |
| 70 | Krause2016SeekAView | 0.00 | 0.12 | 0.00 | 0.00 | 0.00 | 0.88 | 0.00 | 0.00 | 0.00 | 0.00 |
| 71 | Krause2016Using | 0.16 | 0.00 | 0.00 | 0.00 | 0.24 | 0.00 | 0.00 | 0.00 | 0.00 | 0.60 |
| 72 | Rieck2016Exploring | 0.00 | 0.00 | 0.00 | 0.31 | 0.00 | 0.68 | 0.00 | 0.00 | 0.00 | 0.00 |
| 73 | Stahnke2016Probing | 0.15 | 0.00 | 0.00 | 0.04 | 0.52 | 0.23 | 0.06 | 0.00 | 0.00 | 0.00 |
| 74 | Turkay2016Enhancing | 0.31 | 0.21 | 0.00 | 0.00 | 0.00 | 0.00 | 0.00 | 0.00 | 0.00 | 0.49 |
| 75 | Xia2016DimScanner | 0.00 | 0.30 | 0.00 | 0.00 | 0.00 | 0.16 | 0.03 | 0.00 | 0.51 | 0.00 |
| 76 | Zhang2016AVisual | 0.59 | 0.41 | 0.00 | 0.00 | 0.00 | 0.00 | 0.00 | 0.00 | 0.00 | 0.00 |
| 77 | Zhao2016Manifold | 0.00 | 0.00 | 0.00 | 0.67 | 0.33 | 0.00 | 0.00 | 0.00 | 0.00 | 0.00 |
| 78 | Zhou2016Dimension | 0.00 | 0.06 | 0.00 | 0.00 | 0.00 | 0.94 | 0.00 | 0.00 | 0.00 | 0.00 |
| 79 | Badam2017Steering | 0.16 | 0.00 | 0.00 | 0.00 | 0.00 | 0.46 | 0.27 | 0.10 | 0.01 | 0.00 |
| 80 | Bernard2017Combining | 0.00 | 0.00 | 0.00 | 0.00 | 0.00 | 0.69 | 0.13 | 0.18 | 0.00 | 0.00 |
| 81 | Chae2017Visualization | 0.00 | 0.00 | 0.57 | 0.06 | 0.33 | 0.00 | 0.00 | 0.00 | 0.00 | 0.04 |
| 82 | Cypko2017Visual | 0.21 | 0.13 | 0.00 | 0.33 | 0.00 | 0.00 | 0.00 | 0.00 | 0.10 | 0.23 |
| 83 | Jackle2017Pattern | 0.00 | 0.13 | 0.00 | 0.00 | 0.00 | 0.84 | 0.02 | 0.00 | 0.00 | 0.00 |
| 84 | Jiang2017Interactive | 0.00 | 0.00 | 0.11 | 0.00 | 0.09 | 0.68 | 0.00 | 0.00 | 0.00 | 0.11 |
| 85 | Krause2017AWorkflow | 0.80 | 0.13 | 0.00 | 0.00 | 0.00 | 0.00 | 0.00 | 0.00 | 0.00 | 0.06 |
| 86 | Kwon2017AxiSketcher | 0.00 | 0.11 | 0.00 | 0.00 | 0.54 | 0.25 | 0.06 | 0.00 | 0.00 | 0.04 |
| 87 | Liu2017Towards | 0.00 | 0.00 | 0.44 | 0.00 | 0.51 | 0.06 | 0.00 | 0.00 | 0.00 | 0.00 |
| 88 | Ma2017EasySVM | 0.00 | 0.03 | 0.00 | 0.00 | 0.93 | 0.00 | 0.00 | 0.00 | 0.00 | 0.04 |
| 89 | Micallef2017Interactive | 0.65 | 0.00 | 0.00 | 0.00 | 0.08 | 0.16 | 0.00 | 0.00 | 0.03 | 0.08 |
| 90 | Ming2017Understanding | 0.00 | 0.00 | 0.12 | 0.03 | 0.00 | 0.00 | 0.00 | 0.00 | 0.86 | 0.00 |
| 91 | Peltonen2017Negative | 0.17 | 0.00 | 0.00 | 0.00 | 0.00 | 0.83 | 0.00 | 0.00 | 0.00 | 0.00 |
| 92 | Rauber2017Visualizing | 0.00 | 0.00 | 0.03 | 0.00 | 0.97 | 0.00 | 0.00 | 0.00 | 0.00 | 0.00 |
| 93 | Ren2017Squares | 0.05 | 0.00 | 0.00 | 0.00 | 0.46 | 0.00 | 0.00 | 0.00 | 0.00 | 0.50 |
| 94 | Schneider2017Visual | 0.00 | 0.21 | 0.00 | 0.00 | 0.57 | 0.11 | 0.00 | 0.00 | 0.00 | 0.11 |
| 95 | Shao2017Interactive | 0.00 | 0.15 | 0.00 | 0.00 | 0.75 | 0.10 | 0.00 | 0.00 | 0.00 | 0.00 |
| 96 | Strezoski2017Plug | 0.00 | 0.00 | 0.66 | 0.02 | 0.32 | 0.00 | 0.00 | 0.00 | 0.00 | 0.00 |
| 97 | Sun2017Label | 0.32 | 0.00 | 0.00 | 0.00 | 0.00 | 0.08 | 0.00 | 0.45 | 0.00 | 0.15 |
| 98 | Tamagnini2017Interpreting | 0.42 | 0.00 | 0.00 | 0.00 | 0.07 | 0.08 | 0.00 | 0.29 | 0.01 | 0.13 |
| 99 | Wang2017Linear | 0.00 | 0.00 | 0.00 | 0.00 | 0.43 | 0.57 | 0.00 | 0.00 | 0.00 | 0.00 |
| 100 | Wongsuphasawat2018Visualizing | 0.00 | 0.00 | 0.10 | 0.00 | 0.33 | 0.00 | 0.00 | 0.00 | 0.44 | 0.13 |
| 101 | Zeng2017CNNComparator | 0.00 | 0.00 | 0.24 | 0.00 | 0.67 | 0.00 | 0.00 | 0.00 | 0.09 | 0.00 |
| 102 | Alsallakh2018Do | 0.00 | 0.00 | 0.10 | 0.00 | 0.90 | 0.00 | 0.00 | 0.00 | 0.00 | 0.00 |
| 103 | Alvarez2018On | 0.19 | 0.00 | 0.00 | 0.00 | 0.81 | 0.00 | 0.00 | 0.00 | 0.00 | 0.00 |
| 104 | Bernard2018Towards | 0.00 | 0.00 | 0.00 | 0.00 | 0.00 | 0.06 | 0.00 | 0.94 | 0.00 | 0.00 |
| 105 | Cashman2018RNNbow | 0.00 | 0.05 | 0.76 | 0.00 | 0.14 | 0.00 | 0.00 | 0.00 | 0.05 | 0.01 |
| 106 | Cavallo2018AVisual | 0.00 | 0.10 | 0.00 | 0.00 | 0.84 | 0.06 | 0.00 | 0.00 | 0.00 | 0.00 |
| 107 | Cavallo2018Track | 0.00 | 0.00 | 0.00 | 0.00 | 0.39 | 0.00 | 0.00 | 0.06 | 0.00 | 0.56 |
| 108 | Chegini2018Interactive | 0.00 | 0.00 | 0.00 | 0.00 | 0.00 | 1.00 | 0.00 | 0.00 | 0.00 | 0.00 |
| 109 | Chen2018AnchorViz | 0.11 | 0.00 | 0.00 | 0.00 | 0.00 | 0.60 | 0.00 | 0.19 | 0.00 | 0.10 |
| 110 | Cutura2018VisCoDeR | 0.00 | 0.00 | 0.00 | 0.21 | 0.76 | 0.00 | 0.03 | 0.00 | 0.00 | 0.00 |
| 111 | ElAssady2018ThreadRecostructor | 0.00 | 0.00 | 0.00 | 0.03 | 0.00 | 0.08 | 0.00 | 0.06 | 0.03 | 0.79 |
| 112 | Jentner2018Minions | 0.26 | 0.00 | 0.01 | 0.02 | 0.03 | 0.00 | 0.02 | 0.32 | 0.00 | 0.33 |
| 113 | Kahng2018ActiVis | 0.00 | 0.03 | 0.15 | 0.00 | 0.47 | 0.00 | 0.00 | 0.14 | 0.02 | 0.19 |
| 114 | Karer2018Panning | 0.00 | 0.00 | 0.00 | 0.00 | 0.00 | 0.00 | 0.64 | 0.04 | 0.00 | 0.32 |
| 115 | Kauer2018Mapping | 0.04 | 0.00 | 0.35 | 0.00 | 0.00 | 0.19 | 0.00 | 0.07 | 0.00 | 0.34 |
| 116 | Krause2018AUser | 0.91 | 0.00 | 0.00 | 0.00 | 0.02 | 0.00 | 0.00 | 0.07 | 0.00 | 0.00 |
| 117 | Kwon2018Clustervision | 0.00 | 0.00 | 0.00 | 0.00 | 0.00 | 0.87 | 0.00 | 0.00 | 0.00 | 0.13 |
| 118 | Laugel2018Defining | 0.05 | 0.03 | 0.00 | 0.00 | 0.92 | 0.00 | 0.00 | 0.00 | 0.00 | 0.00 |
| 119 | Li2018EmbeddingVis | 0.00 | 0.02 | 0.00 | 0.54 | 0.00 | 0.00 | 0.00 | 0.00 | 0.44 | 0.00 |
| 120 | Lin2018RCLens | 0.00 | 0.00 | 0.00 | 0.00 | 0.00 | 0.09 | 0.00 | 0.11 | 0.80 | 0.00 |

Table 3: The topic modeling results for our survey (continued).

| # | Technique | Topic_1 | Topic_2 | Topic_3 | Topic_4 | Topic_5 | Topic_6 | Topic_7 | Topic_8 | Topic_9 | Topic_10 |
|---|---|---|---|---|---|---|---|---|---|---|---|
| 121 | Liu2018Analyzing | 0.00 | 0.00 | 0.71 | 0.00 | 0.29 | 0.00 | 0.00 | 0.00 | 0.00 | 0.00 |
| 122 | Liu2018AnalyzingtheT | 0.00 | 0.00 | 0.71 | 0.00 | 0.27 | 0.00 | 0.00 | 0.00 | 0.02 | 0.00 |
| 123 | Liu2018DeepTracker | 0.00 | 0.00 | 0.70 | 0.00 | 0.30 | 0.00 | 0.00 | 0.00 | 0.00 | 0.00 |
| 124 | Liu2018Visual | 0.00 | 0.78 | 0.12 | 0.00 | 0.00 | 0.00 | 0.00 | 0.00 | 0.10 | 0.00 |
| 125 | Liu2018VisualExploration | 0.00 | 0.00 | 0.00 | 0.53 | 0.15 | 0.02 | 0.00 | 0.01 | 0.29 | 0.00 |
| 126 | Muhlbacher2018TreePOD | 0.00 | 1.00 | 0.00 | 0.00 | 0.00 | 0.00 | 0.00 | 0.00 | 0.00 | 0.00 |
| 127 | Nie2018Visualizing | 0.00 | 0.08 | 0.38 | 0.00 | 0.26 | 0.00 | 0.00 | 0.00 | 0.27 | 0.00 |
| 128 | Olah2018The | 0.05 | 0.00 | 0.24 | 0.03 | 0.51 | 0.00 | 0.00 | 0.18 | 0.00 | 0.00 |
| 129 | Pezzotti2018DeepEyes | 0.00 | 0.00 | 0.69 | 0.00 | 0.31 | 0.00 | 0.00 | 0.00 | 0.00 | 0.00 |
| 130 | Rauber2018Projections | 0.00 | 0.00 | 0.00 | 0.00 | 1.00 | 0.00 | 0.00 | 0.00 | 0.00 | 0.00 |
| 131 | Sacha2018SOMFlow | 0.00 | 0.02 | 0.00 | 0.00 | 0.00 | 0.14 | 0.78 | 0.00 | 0.06 | 0.00 |
| 132 | Schall2018Visualization | 0.00 | 0.00 | 0.40 | 0.00 | 0.59 | 0.00 | 0.00 | 0.00 | 0.00 | 0.00 |
| 133 | Schneider2018Integrating | 0.00 | 0.33 | 0.00 | 0.00 | 0.30 | 0.16 | 0.00 | 0.00 | 0.08 | 0.13 |
| 134 | Sehgal2018Visual | 0.00 | 0.19 | 0.00 | 0.00 | 0.11 | 0.13 | 0.00 | 0.00 | 0.00 | 0.56 |
| 135 | Sevastjanova2018Going | 0.19 | 0.03 | 0.11 | 0.00 | 0.00 | 0.14 | 0.00 | 0.52 | 0.00 | 0.01 |
| 136 | Sherkat2018Interactive | 0.00 | 0.00 | 0.00 | 0.00 | 0.00 | 1.00 | 0.00 | 0.00 | 0.00 | 0.00 |
| 137 | Strobelt2018LSTMVis | 0.00 | 0.23 | 0.36 | 0.04 | 0.00 | 0.00 | 0.00 | 0.20 | 0.15 | 0.02 |
| 138 | Sun2018FraudVis | 0.00 | 0.00 | 0.03 | 0.00 | 0.00 | 0.00 | 0.00 | 0.00 | 0.86 | 0.11 |
| 139 | Thiagarajan2018Exploring | 0.00 | 0.00 | 0.00 | 0.10 | 0.86 | 0.04 | 0.00 | 0.00 | 0.00 | 0.00 |
| 140 | Vogogias2018BayesPiles | 0.05 | 0.80 | 0.00 | 0.00 | 0.00 | 0.00 | 0.00 | 0.13 | 0.02 | 0.00 |
| 141 | Wang2018GANViz | 0.00 | 0.00 | 0.53 | 0.00 | 0.47 | 0.00 | 0.00 | 0.00 | 0.00 | 0.00 |
| 142 | Wang2018The | 0.00 | 0.00 | 0.00 | 0.00 | 0.00 | 0.28 | 0.72 | 0.00 | 0.00 | 0.00 |
| 143 | Xia2018LDSScanner | 0.00 | 0.03 | 0.00 | 0.41 | 0.27 | 0.30 | 0.00 | 0.00 | 0.00 | 0.00 |
| 144 | Yan2018Homology | 0.00 | 0.00 | 0.00 | 1.00 | 0.00 | 0.00 | 0.00 | 0.00 | 0.00 | 0.00 |
| 145 | Zhao2018SkyLens | 0.06 | 0.70 | 0.00 | 0.00 | 0.00 | 0.04 | 0.00 | 0.00 | 0.20 | 0.00 |
| 146 | Arendt2019Towards | 0.00 | 0.00 | 0.00 | 0.00 | 0.00 | 0.45 | 0.00 | 0.37 | 0.00 | 0.17 |
| 147 | Bernard2019Visual | 0.00 | 0.00 | 0.00 | 0.00 | 0.00 | 0.08 | 0.00 | 0.92 | 0.00 | 0.00 |
| 148 | Caballero2019V | 0.24 | 0.00 | 0.17 | 0.00 | 0.56 | 0.00 | 0.00 | 0.00 | 0.00 | 0.03 |
| 149 | Cabrera2019FairVis | 0.12 | 0.00 | 0.00 | 0.00 | 0.00 | 0.02 | 0.00 | 0.00 | 0.00 | 0.86 |
| 150 | Cashman2019AUser | 0.03 | 0.01 | 0.00 | 0.00 | 0.17 | 0.01 | 0.00 | 0.00 | 0.00 | 0.78 |
| 151 | Cavallo2019Clustrophile2 | 0.05 | 0.00 | 0.00 | 0.00 | 0.00 | 0.91 | 0.00 | 0.00 | 0.04 | 0.00 |
| 152 | Chegini2019Interactive | 0.00 | 0.00 | 0.00 | 0.00 | 0.00 | 0.82 | 0.00 | 0.18 | 0.00 | 0.00 |
| 153 | Chen2019LDA | 0.00 | 0.00 | 0.03 | 0.00 | 0.00 | 0.91 | 0.00 | 0.00 | 0.06 | 0.00 |
| 154 | Das2019BEAMES | 0.00 | 0.03 | 0.00 | 0.00 | 0.34 | 0.32 | 0.00 | 0.00 | 0.00 | 0.30 |
| 155 | Gil2019Towards | 0.00 | 0.00 | 0.00 | 0.00 | 0.00 | 0.00 | 0.00 | 0.00 | 0.00 | 1.00 |
| 156 | Guo2019Visualizing | 0.38 | 0.00 | 0.00 | 0.00 | 0.00 | 0.00 | 0.00 | 0.00 | 0.53 | 0.09 |
| 157 | Hamid2019Visual | 0.00 | 0.00 | 0.00 | 0.00 | 1.00 | 0.00 | 0.00 | 0.00 | 0.00 | 0.00 |
| 158 | Hohman2019Gamut | 0.80 | 0.00 | 0.00 | 0.00 | 0.00 | 0.00 | 0.00 | 0.02 | 0.00 | 0.18 |
| 159 | Hohman2019TeleGam | 0.46 | 0.00 | 0.00 | 0.01 | 0.00 | 0.00 | 0.00 | 0.36 | 0.00 | 0.17 |
| 160 | Hollt2019Focus | 0.00 | 0.04 | 0.00 | 0.27 | 0.58 | 0.10 | 0.00 | 0.00 | 0.00 | 0.00 |
| 161 | Huang2019GBRTVis | 0.00 | 0.87 | 0.03 | 0.00 | 0.06 | 0.02 | 0.02 | 0.00 | 0.00 | 0.00 |
| 162 | Janik2019Interpreting | 0.02 | 0.00 | 0.41 | 0.00 | 0.33 | 0.02 | 0.00 | 0.07 | 0.00 | 0.15 |
| 163 | Ji2019Visual | 0.00 | 0.00 | 0.03 | 0.74 | 0.00 | 0.23 | 0.00 | 0.00 | 0.00 | 0.00 |
| 164 | Kahng2019GAN | 0.00 | 0.00 | 1.00 | 0.00 | 0.00 | 0.00 | 0.00 | 0.00 | 0.00 | 0.00 |
| 165 | Kinkeldey2019Towards | 0.22 | 0.00 | 0.00 | 0.00 | 0.00 | 0.63 | 0.07 | 0.00 | 0.00 | 0.07 |
| 166 | Kwon2019RetainVis | 0.00 | 0.00 | 0.06 | 0.03 | 0.00 | 0.00 | 0.00 | 0.00 | 0.24 | 0.67 |
| 167 | Liu2019Latent | 0.00 | 0.01 | 0.00 | 0.23 | 0.21 | 0.02 | 0.00 | 0.03 | 0.50 | 0.00 |
| 168 | Liu2019NLIZE | 0.00 | 0.00 | 0.05 | 0.15 | 0.00 | 0.00 | 0.00 | 0.07 | 0.72 | 0.00 |
| 169 | Madsen2019Visualizing | 0.04 | 0.00 | 0.41 | 0.00 | 0.00 | 0.00 | 0.41 | 0.00 | 0.14 | 0.00 |
| 170 | Ming2019Interpretable | 0.02 | 0.00 | 0.14 | 0.04 | 0.03 | 0.00 | 0.00 | 0.03 | 0.15 | 0.58 |
| 171 | Ming2019RuleMatrix | 0.00 | 0.00 | 0.00 | 0.00 | 0.16 | 0.00 | 0.00 | 0.00 | 0.10 | 0.74 |
| 172 | Murugesan2019DeepCompare | 0.00 | 0.00 | 0.10 | 0.00 | 0.46 | 0.00 | 0.00 | 0.13 | 0.08 | 0.23 |
| 173 | Park2019ComDia | 0.00 | 0.00 | 0.00 | 0.00 | 0.75 | 0.00 | 0.00 | 0.00 | 0.00 | 0.25 |
| 174 | Roesch2019Visualization | 0.00 | 0.00 | 0.22 | 0.00 | 0.58 | 0.00 | 0.00 | 0.00 | 0.20 | 0.00 |
| 175 | Sacha2019VIS4ML | 0.00 | 0.03 | 0.51 | 0.00 | 0.00 | 0.00 | 0.06 | 0.11 | 0.01 | 0.28 |
| 176 | Saldanha2019ReLVis | 0.00 | 0.00 | 0.76 | 0.00 | 0.10 | 0.00 | 0.00 | 0.00 | 0.00 | 0.14 |
| 177 | Sawatzky2019Visualizing | 0.00 | 0.15 | 0.49 | 0.10 | 0.00 | 0.00 | 0.00 | 0.20 | 0.06 | 0.00 |
| 178 | Steinparz2019Visualization | 0.00 | 0.00 | 0.00 | 0.00 | 0.10 | 0.09 | 0.08 | 0.73 | 0.00 | 0.00 |
| 179 | Strobelt2019Seq2seq | 0.00 | 0.00 | 0.14 | 0.30 | 0.00 | 0.00 | 0.00 | 0.04 | 0.46 | 0.06 |
| 180 | Tyagi2019ICE | 0.00 | 0.19 | 0.00 | 0.00 | 0.06 | 0.00 | 0.47 | 0.00 | 0.01 | 0.26 |
| 181 | Vig2019A | 0.00 | 0.00 | 0.00 | 0.95 | 0.05 | 0.00 | 0.00 | 0.00 | 0.00 | 0.00 |
| 182 | Wang2019ATMSeer | 0.00 | 0.00 | 0.00 | 0.03 | 0.00 | 0.00 | 0.00 | 0.00 | 0.00 | 0.97 |
| 183 | Wang2019DeepVID | 0.00 | 0.00 | 0.09 | 0.00 | 0.84 | 0.00 | 0.00 | 0.00 | 0.06 | 0.00 |
| 184 | Wang2019DQNViz | 0.00 | 0.00 | 1.00 | 0.00 | 0.00 | 0.00 | 0.00 | 0.00 | 0.00 | 0.00 |
| 185 | Wang2019High | 0.00 | 0.00 | 0.00 | 0.00 | 0.00 | 1.00 | 0.00 | 0.00 | 0.00 | 0.00 |
| 186 | Xu2019EnsembleLens | 0.00 | 0.00 | 0.00 | 0.00 | 0.00 | 0.29 | 0.02 | 0.00 | 0.69 | 0.00 |
| 187 | Zhang2019Manifold | 0.11 | 0.02 | 0.00 | 0.00 | 0.40 | 0.00 | 0.00 | 0.05 | 0.34 | 0.08 |
| 188 | Zhao2019FeatureExplorer | 0.00 | 0.34 | 0.00 | 0.00 | 0.27 | 0.00 | 0.00 | 0.00 | 0.14 | 0.26 |
| 189 | Zhao2019iForest | 0.00 | 0.25 | 0.00 | 0.00 | 0.00 | 0.00 | 0.00 | 0.00 | 0.57 | 0.17 |
| 190 | Zhao2019Oui | 0.01 | 0.00 | 0.00 | 0.00 | 0.00 | 0.18 | 0.00 | 0.00 | 0.81 | 0.00 |

Table 4: The topic modeling results for our survey (continued).

| # | Technique | Topic_1 | Topic_2 | Topic_3 | Topic_4 | Topic_5 | Topic_6 | Topic_7 | Topic_8 | Topic_9 | Topic_10 |
|---|---|---|---|---|---|---|---|---|---|---|---|
| 191 | Ahn2019FairSight | 0.82 | 0.00 | 0.00 | 0.09 | 0.00 | 0.00 | 0.00 | 0.00 | 0.09 | 0.00 |
| 192 | Bauerle2020Classifier | 0.00 | 0.00 | 0.00 | 0.00 | 0.61 | 0.00 | 0.00 | 0.39 | 0.00 | 0.00 |
| 193 | Borland2019Selection | 0.02 | 0.38 | 0.00 | 0.00 | 0.00 | 0.01 | 0.00 | 0.00 | 0.00 | 0.58 |
| 194 | Cashman2019Ablate | 0.00 | 0.00 | 0.09 | 0.00 | 0.36 | 0.00 | 0.00 | 0.00 | 0.00 | 0.55 |
| 195 | Chatzimparmpas2020t-viSNE | 0.01 | 0.06 | 0.00 | 0.00 | 0.50 | 0.35 | 0.03 | 0.00 | 0.05 | 0.00 |
| 196 | Collaris2020ExplainExplore | 0.28 | 0.06 | 0.00 | 0.00 | 0.50 | 0.00 | 0.00 | 0.00 | 0.04 | 0.12 |
| 197 | Das2020QUESTO | 0.00 | 0.00 | 0.00 | 0.00 | 0.00 | 0.04 | 0.00 | 0.82 | 0.00 | 0.14 |
| 198 | Fujiwara2019Supporting | 0.00 | 0.00 | 0.00 | 0.66 | 0.00 | 0.34 | 0.00 | 0.00 | 0.00 | 0.00 |
| 199 | Fujiwara2020An | 0.00 | 0.00 | 0.00 | 0.18 | 0.00 | 0.00 | 0.82 | 0.00 | 0.00 | 0.00 |
| 200 | Gehrmann2019Visual | 0.15 | 0.00 | 0.25 | 0.22 | 0.00 | 0.00 | 0.00 | 0.11 | 0.00 | 0.28 |
| 201 | Gleicher2020Boxer | 0.03 | 0.04 | 0.00 | 0.00 | 0.62 | 0.02 | 0.00 | 0.08 | 0.00 | 0.21 |
| 202 | Gomez2020ViCE | 0.60 | 0.00 | 0.00 | 0.00 | 0.00 | 0.00 | 0.00 | 0.07 | 0.00 | 0.33 |
| 203 | Gortler2020Uncertainty | 0.00 | 0.00 | 0.00 | 0.00 | 0.24 | 0.00 | 0.76 | 0.00 | 0.00 | 0.00 |
| 204 | Hazarika2019NNVA | 0.00 | 0.00 | 0.01 | 0.00 | 0.99 | 0.00 | 0.00 | 0.00 | 0.00 | 0.00 |
| 205 | He2020DynamicsExplorer | 0.00 | 0.00 | 0.91 | 0.02 | 0.00 | 0.05 | 0.02 | 0.00 | 0.00 | 0.00 |
| 206 | Hohman2020Summit | 0.00 | 0.00 | 0.16 | 0.00 | 0.84 | 0.00 | 0.00 | 0.00 | 0.00 | 0.00 |
| 207 | Hohman2020Understanding | 0.00 | 0.02 | 0.00 | 0.00 | 0.00 | 0.00 | 0.00 | 0.18 | 0.05 | 0.75 |
| 208 | Jaunet2020DRLViz | 0.00 | 0.00 | 0.87 | 0.00 | 0.01 | 0.10 | 0.00 | 0.00 | 0.00 | 0.00 |
| 209 | Johnson2020NJM | 0.45 | 0.00 | 0.05 | 0.13 | 0.08 | 0.00 | 0.00 | 0.17 | 0.12 | 0.00 |
| 210 | Jonsson2020Visual | 0.00 | 0.00 | 0.00 | 0.00 | 1.00 | 0.00 | 0.00 | 0.00 | 0.00 | 0.00 |
| 211 | Khayat2019VASSL | 0.00 | 0.00 | 0.00 | 0.00 | 0.00 | 0.37 | 0.00 | 0.12 | 0.47 | 0.03 |
| 212 | Lekschas2020PEAX | 0.00 | 0.00 | 0.03 | 0.00 | 0.15 | 0.66 | 0.00 | 0.16 | 0.00 | 0.00 |
| 213 | Li2020A | 0.25 | 0.39 | 0.08 | 0.21 | 0.03 | 0.00 | 0.00 | 0.00 | 0.00 | 0.04 |
| 214 | Li2020Visualizing | 0.00 | 0.00 | 0.03 | 0.00 | 0.97 | 0.00 | 0.00 | 0.00 | 0.00 | 0.00 |
| 215 | Li2021Inspecting | 0.00 | 0.00 | 0.67 | 0.00 | 0.00 | 0.00 | 0.00 | 0.00 | 0.33 | 0.00 |
| 216 | Ma2019Explaining | 0.00 | 0.00 | 0.04 | 0.00 | 0.56 | 0.00 | 0.00 | 0.23 | 0.12 | 0.05 |
| 217 | Ming2019ProtoSteer | 0.00 | 0.00 | 0.08 | 0.01 | 0.00 | 0.00 | 0.00 | 0.00 | 0.36 | 0.54 |
| 218 | Pan2020RCAnalyzer | 0.00 | 0.02 | 0.00 | 0.00 | 0.00 | 0.00 | 0.00 | 0.00 | 0.98 | 0.00 |
| 219 | Puhringer2020InstanceFlow | 0.00 | 0.00 | 0.00 | 0.00 | 0.79 | 0.00 | 0.00 | 0.15 | 0.06 | 0.00 |
| 220 | Sahoo2020Visually | 0.00 | 0.63 | 0.00 | 0.02 | 0.20 | 0.00 | 0.00 | 0.01 | 0.12 | 0.02 |
| 221 | Schlegel2020Towards | 0.03 | 0.00 | 0.00 | 0.00 | 0.63 | 0.00 | 0.00 | 0.12 | 0.15 | 0.07 |
| 222 | Shen2020Visual | 0.00 | 0.00 | 0.05 | 0.00 | 0.00 | 0.00 | 0.00 | 0.00 | 0.95 | 0.00 |
| 223 | Shrivastava2020iSeqL | 0.06 | 0.00 | 0.00 | 0.00 | 0.00 | 0.00 | 0.00 | 0.81 | 0.00 | 0.13 |
| 224 | Spinner2020explAIner | 0.09 | 0.00 | 0.09 | 0.00 | 0.00 | 0.00 | 0.12 | 0.52 | 0.00 | 0.18 |
| 225 | Sun2020DFSeer | 0.04 | 0.00 | 0.00 | 0.00 | 0.00 | 0.00 | 0.00 | 0.00 | 0.90 | 0.05 |
| 226 | Tenney2020The | 0.03 | 0.00 | 0.00 | 0.13 | 0.00 | 0.00 | 0.00 | 0.68 | 0.00 | 0.16 |
| 227 | Wang2020ConceptExplorer | 0.00 | 0.69 | 0.13 | 0.00 | 0.00 | 0.00 | 0.00 | 0.08 | 0.10 | 0.00 |
| 228 | Wang2020SCANViz | 0.00 | 0.00 | 0.35 | 0.00 | 0.19 | 0.00 | 0.00 | 0.01 | 0.44 | 0.00 |
| 229 | Wang2020Visual | 0.00 | 0.00 | 0.23 | 0.00 | 0.00 | 0.00 | 0.00 | 0.00 | 0.77 | 0.00 |
| 230 | Wang2021Visual | 0.86 | 0.13 | 0.00 | 0.00 | 0.00 | 0.00 | 0.00 | 0.00 | 0.00 | 0.00 |
| 231 | Weidele2020AutoAIViz | 0.34 | 0.00 | 0.00 | 0.03 | 0.00 | 0.00 | 0.00 | 0.00 | 0.00 | 0.62 |
| 232 | Wexler2019The | 0.14 | 0.00 | 0.00 | 0.00 | 0.20 | 0.00 | 0.00 | 0.00 | 0.00 | 0.66 |
| 233 | Yang2020Diagnosing | 0.00 | 0.00 | 0.14 | 0.00 | 0.02 | 0.01 | 0.79 | 0.00 | 0.03 | 0.00 |
| 234 | Yang2020How | 0.82 | 0.09 | 0.00 | 0.00 | 0.03 | 0.00 | 0.00 | 0.06 | 0.00 | 0.00 |
| 235 | Alharbi2021VNLP | 0.00 | 0.00 | 0.28 | 0.47 | 0.00 | 0.00 | 0.00 | 0.15 | 0.00 | 0.11 |
| 236 | Bernard2021A | 0.00 | 0.02 | 0.00 | 0.00 | 0.00 | 0.06 | 0.00 | 0.93 | 0.00 | 0.00 |
| 237 | Bernard2021ProSeCo | 0.00 | 0.15 | 0.00 | 0.00 | 0.67 | 0.09 | 0.09 | 0.00 | 0.00 | 0.00 |
| 238 | Bian2021Semantic | 0.37 | 0.00 | 0.00 | 0.06 | 0.03 | 0.10 | 0.40 | 0.05 | 0.00 | 0.00 |
| 239 | Bibal2021IXVC | 0.15 | 0.23 | 0.00 | 0.00 | 0.09 | 0.52 | 0.00 | 0.00 | 0.00 | 0.00 |
| 240 | Caballero2021PerSleep | 0.53 | 0.00 | 0.00 | 0.00 | 0.34 | 0.00 | 0.00 | 0.00 | 0.00 | 0.13 |
| 241 | Cao2021SHIM | 0.00 | 0.08 | 0.00 | 0.00 | 0.00 | 0.78 | 0.00 | 0.00 | 0.00 | 0.13 |
| 242 | Cashman2021CAVA | 0.16 | 0.44 | 0.00 | 0.00 | 0.00 | 0.00 | 0.00 | 0.06 | 0.00 | 0.35 |
| 243 | Chatzimparmpas2021StackGenVis | 0.00 | 0.08 | 0.00 | 0.00 | 0.11 | 0.19 | 0.00 | 0.00 | 0.12 | 0.50 |
| 244 | Chatzimparmpas2021VisEvol | 0.00 | 0.00 | 0.00 | 0.00 | 0.03 | 0.69 | 0.00 | 0.00 | 0.00 | 0.28 |
| 245 | Chen2021Interactive | 0.00 | 0.00 | 0.00 | 0.00 | 0.12 | 0.02 | 0.00 | 0.05 | 0.80 | 0.00 |
| 246 | Chen2021OoDAnalyzer | 0.00 | 0.00 | 0.39 | 0.00 | 0.36 | 0.01 | 0.00 | 0.00 | 0.24 | 0.00 |
| 247 | Cheng2021DECE | 0.41 | 0.07 | 0.00 | 0.00 | 0.06 | 0.00 | 0.00 | 0.00 | 0.11 | 0.35 |
| 248 | Chotisarn2021Deep | 0.00 | 0.00 | 0.09 | 0.03 | 0.13 | 0.17 | 0.00 | 0.00 | 0.09 | 0.49 |
| 249 | Das2021CACTUS | 0.00 | 0.00 | 0.00 | 0.00 | 0.00 | 0.00 | 0.00 | 0.98 | 0.00 | 0.02 |
| 250 | Das2021Geono | 0.12 | 0.00 | 0.00 | 0.00 | 0.00 | 0.81 | 0.00 | 0.00 | 0.00 | 0.08 |
| 251 | Deng2021RISSAD | 0.00 | 0.00 | 0.00 | 0.00 | 0.07 | 0.33 | 0.10 | 0.00 | 0.27 | 0.23 |
| 252 | Espadoto2021Self | 0.00 | 0.00 | 0.00 | 0.00 | 0.73 | 0.27 | 0.00 | 0.00 | 0.00 | 0.00 |
| 253 | Espadoto2021UnProjection | 0.00 | 0.00 | 0.00 | 0.00 | 1.00 | 0.00 | 0.00 | 0.00 | 0.00 | 0.00 |
| 254 | Francoise2021Marcelle | 0.00 | 0.00 | 0.06 | 0.00 | 0.00 | 0.00 | 0.00 | 0.00 | 0.00 | 0.94 |
| 255 | Garcia2021Visual | 0.00 | 0.46 | 0.25 | 0.00 | 0.13 | 0.00 | 0.00 | 0.04 | 0.12 | 0.00 |
| 256 | Gomez2021AdViCE | 0.52 | 0.06 | 0.00 | 0.00 | 0.15 | 0.00 | 0.00 | 0.00 | 0.00 | 0.26 |
| 257 | Guo2021Interpretable | 0.00 | 0.00 | 0.00 | 0.00 | 0.00 | 0.00 | 0.00 | 0.00 | 1.00 | 0.00 |
| 258 | Han2021IVDAS | 0.00 | 0.00 | 0.58 | 0.00 | 0.42 | 0.00 | 0.00 | 0.00 | 0.00 | 0.00 |
| 259 | Hepenstal2021Developing | 0.29 | 0.00 | 0.47 | 0.00 | 0.00 | 0.00 | 0.00 | 0.24 | 0.00 | 0.00 |
| 260 | Hinterreiter2021Projection | 0.00 | 0.00 | 0.00 | 0.06 | 0.18 | 0.04 | 0.00 | 0.71 | 0.00 | 0.00 |

Table 5: The topic modeling results for our survey (continued).

| # | Technique | Topic_1 | Topic_2 | Topic_3 | Topic_4 | Topic_5 | Topic_6 | Topic_7 | Topic_8 | Topic_9 | Topic_10 |
|---|---|---|---|---|---|---|---|---|---|---|---|
| 261 | Hoque2021Outcome | 0.89 | 0.03 | 0.00 | 0.00 | 0.00 | 0.00 | 0.00 | 0.00 | 0.00 | 0.07 |
| 262 | Huang2021A | 0.00 | 0.00 | 0.06 | 0.00 | 0.55 | 0.00 | 0.00 | 0.00 | 0.34 | 0.05 |
| 263 | Ji2021USEVis | 0.00 | 0.00 | 0.00 | 1.00 | 0.00 | 0.00 | 0.00 | 0.00 | 0.00 | 0.00 |
| 264 | Jo2021ProReveal | 0.49 | 0.00 | 0.00 | 0.00 | 0.01 | 0.00 | 0.42 | 0.02 | 0.00 | 0.05 |
| 265 | Kim2021Learn | 0.57 | 0.00 | 0.36 | 0.00 | 0.00 | 0.00 | 0.00 | 0.07 | 0.00 | 0.00 |
| 266 | Knittel2021Visual | 0.02 | 0.53 | 0.00 | 0.00 | 0.39 | 0.06 | 0.00 | 0.00 | 0.00 | 0.00 |
| 267 | Krause2021Visual | 0.00 | 0.05 | 0.00 | 0.00 | 0.03 | 0.38 | 0.00 | 0.48 | 0.06 | 0.00 |
| 268 | Lee2021FedNLP | 0.04 | 0.00 | 0.25 | 0.12 | 0.00 | 0.00 | 0.00 | 0.10 | 0.00 | 0.49 |
| 269 | Li2021CNNPruner | 0.00 | 0.03 | 0.30 | 0.00 | 0.02 | 0.00 | 0.65 | 0.00 | 0.00 | 0.00 |
| 270 | Li2021SemanticAxis | 0.00 | 0.15 | 0.00 | 0.04 | 0.00 | 0.00 | 0.82 | 0.00 | 0.00 | 0.00 |
| 271 | Li2021T3 | 0.00 | 0.00 | 0.18 | 0.56 | 0.00 | 0.00 | 0.00 | 0.21 | 0.06 | 0.00 |
| 272 | Lo2021CNERVis | 0.00 | 0.00 | 0.58 | 0.00 | 0.00 | 0.00 | 0.00 | 0.10 | 0.32 | 0.00 |
| 273 | Lu2021Evaluating | 1.00 | 0.00 | 0.00 | 0.00 | 0.00 | 0.00 | 0.00 | 0.00 | 0.00 | 0.00 |
| 274 | Ma2021A | 0.00 | 0.00 | 0.03 | 0.00 | 0.73 | 0.00 | 0.00 | 0.06 | 0.18 | 0.00 |
| 275 | Ma2021Visual | 0.00 | 0.01 | 0.00 | 0.35 | 0.53 | 0.00 | 0.00 | 0.11 | 0.00 | 0.00 |
| 276 | Marcilio2021Contrastive | 0.00 | 0.00 | 0.00 | 0.53 | 0.00 | 0.47 | 0.00 | 0.00 | 0.00 | 0.00 |
| 277 | Marcilio2021Explaining | 0.02 | 0.00 | 0.00 | 0.84 | 0.00 | 0.13 | 0.00 | 0.00 | 0.00 | 0.00 |
| 278 | Marcilio2021ExplorerTree | 0.00 | 0.17 | 0.00 | 0.08 | 0.34 | 0.41 | 0.00 | 0.00 | 0.00 | 0.00 |
| 279 | Meng2021VADAF | 0.00 | 0.00 | 0.90 | 0.00 | 0.10 | 0.00 | 0.00 | 0.00 | 0.00 | 0.00 |
| 280 | Mishra2021Designing | 0.33 | 0.00 | 0.06 | 0.00 | 0.00 | 0.00 | 0.00 | 0.20 | 0.00 | 0.41 |
| 281 | Munz2021Visual | 0.03 | 0.00 | 0.02 | 0.95 | 0.00 | 0.00 | 0.00 | 0.00 | 0.00 | 0.00 |
| 282 | Neto2021Explainable | 0.05 | 0.29 | 0.00 | 0.00 | 0.00 | 0.00 | 0.00 | 0.42 | 0.00 | 0.23 |
| 283 | Nguyen2021XMAP | 0.15 | 0.00 | 0.00 | 0.01 | 0.36 | 0.14 | 0.00 | 0.00 | 0.01 | 0.32 |
| 284 | Nourani2021Anchoring | 1.00 | 0.00 | 0.00 | 0.00 | 0.00 | 0.00 | 0.00 | 0.00 | 0.00 | 0.00 |
| 285 | Ono2021PipelineProfiler | 0.00 | 0.05 | 0.24 | 0.00 | 0.00 | 0.00 | 0.00 | 0.00 | 0.00 | 0.71 |
| 286 | Park2021HyperTendril | 0.00 | 0.00 | 0.11 | 0.46 | 0.00 | 0.00 | 0.00 | 0.00 | 0.00 | 0.42 |
| 287 | Park2021VATUN | 0.08 | 0.00 | 0.31 | 0.00 | 0.62 | 0.00 | 0.00 | 0.00 | 0.00 | 0.00 |
| 288 | Rathore2021TopoAct | 0.00 | 0.00 | 0.00 | 0.22 | 0.78 | 0.00 | 0.00 | 0.00 | 0.00 | 0.00 |
| 289 | Rojo2021AHMoSe | 0.32 | 0.00 | 0.00 | 0.00 | 0.11 | 0.00 | 0.00 | 0.00 | 0.06 | 0.50 |
| 290 | Rostamzadeh2021VERONICA | 0.00 | 0.04 | 0.00 | 0.00 | 0.02 | 0.00 | 0.00 | 0.00 | 0.00 | 0.94 |
| 291 | Roy2021Explainable | 0.60 | 0.08 | 0.16 | 0.00 | 0.08 | 0.00 | 0.00 | 0.08 | 0.00 | 0.00 |
| 292 | Schader2021LayoutExOmizer | 0.00 | 0.00 | 0.00 | 0.00 | 0.27 | 0.00 | 0.72 | 0.00 | 0.00 | 0.00 |
| 293 | Seng2021Visual | 0.00 | 0.00 | 1.00 | 0.00 | 0.00 | 0.00 | 0.00 | 0.00 | 0.00 | 0.00 |
| 294 | Sevastjanova2021Explaining | 0.00 | 0.00 | 0.29 | 0.68 | 0.00 | 0.00 | 0.00 | 0.03 | 0.00 | 0.00 |
| 295 | Sevastjanova2021QuestionComb | 0.00 | 0.00 | 0.00 | 0.00 | 0.00 | 0.00 | 0.00 | 1.00 | 0.00 | 0.00 |
| 296 | Shen2021An | 0.00 | 0.00 | 0.61 | 0.00 | 0.39 | 0.00 | 0.00 | 0.00 | 0.00 | 0.00 |
| 297 | Sperrle2021Learning | 0.00 | 0.00 | 0.15 | 0.00 | 0.00 | 0.55 | 0.00 | 0.13 | 0.00 | 0.16 |
| 298 | Spinner2021Speculative | 0.00 | 0.07 | 0.00 | 0.00 | 0.00 | 0.25 | 0.58 | 0.04 | 0.00 | 0.05 |
| 299 | Strobelt2021LMdiff | 0.00 | 0.00 | 0.00 | 0.39 | 0.00 | 0.00 | 0.00 | 0.35 | 0.25 | 0.00 |
| 300 | Sun2021EvoSets | 0.00 | 0.83 | 0.00 | 0.00 | 0.00 | 0.17 | 0.00 | 0.00 | 0.00 | 0.00 |
| 301 | Suschnigg2021Visual | 0.00 | 0.00 | 0.00 | 0.00 | 0.00 | 0.00 | 0.88 | 0.00 | 0.07 | 0.05 |
| 302 | Tabatabai2021Why | 0.28 | 0.06 | 0.66 | 0.00 | 0.00 | 0.00 | 0.00 | 0.00 | 0.00 | 0.00 |
| 303 | Thomas2021FacetRules | 0.00 | 0.12 | 0.00 | 0.00 | 0.00 | 0.59 | 0.00 | 0.00 | 0.00 | 0.29 |
| 304 | Tian2021Using | 0.01 | 0.00 | 0.00 | 0.00 | 0.98 | 0.00 | 0.00 | 0.00 | 0.00 | 0.00 |
| 305 | Wang2021CNN | 0.08 | 0.00 | 0.92 | 0.00 | 0.00 | 0.00 | 0.00 | 0.00 | 0.00 | 0.00 |
| 306 | Wang2021GAM | 0.00 | 0.00 | 0.00 | 0.00 | 0.00 | 0.00 | 0.00 | 0.00 | 0.00 | 1.00 |
| 307 | Wang2021HypoML | 0.12 | 0.00 | 0.62 | 0.00 | 0.17 | 0.00 | 0.00 | 0.09 | 0.00 | 0.00 |
| 308 | Wang2021Investigating | 0.00 | 0.56 | 0.00 | 0.00 | 0.00 | 0.00 | 0.00 | 0.00 | 0.44 | 0.00 |
| 309 | Wang2021VisualAnalytics | 0.00 | 0.00 | 0.95 | 0.02 | 0.00 | 0.02 | 0.00 | 0.00 | 0.00 | 0.00 |
| 310 | Xia2021GBMVis | 0.00 | 0.00 | 0.11 | 0.00 | 0.00 | 0.00 | 0.00 | 0.00 | 0.00 | 0.89 |
| 311 | Xie2021A | 0.20 | 0.00 | 0.00 | 0.00 | 0.00 | 0.00 | 0.57 | 0.00 | 0.22 | 0.00 |
| 312 | Xie2021Auditing | 0.02 | 0.00 | 0.00 | 0.00 | 0.00 | 0.00 | 0.00 | 0.03 | 0.94 | 0.02 |
| 313 | Xie2021Exploring | 0.00 | 0.57 | 0.00 | 0.05 | 0.05 | 0.33 | 0.00 | 0.00 | 0.00 | 0.00 |
| 314 | Xu2021mTSeer | 0.20 | 0.00 | 0.00 | 0.00 | 0.08 | 0.00 | 0.00 | 0.00 | 0.72 | 0.00 |
| 315 | Yang2021Interactive | 0.00 | 0.23 | 0.02 | 0.01 | 0.00 | 0.61 | 0.00 | 0.00 | 0.10 | 0.02 |
| 316 | Yarlagadda2021DocTable | 0.00 | 0.00 | 0.00 | 0.14 | 0.00 | 0.52 | 0.00 | 0.08 | 0.00 | 0.27 |
| 317 | Yeon2021Visual | 0.00 | 0.22 | 0.00 | 0.00 | 0.00 | 0.00 | 0.00 | 0.00 | 0.64 | 0.14 |
| 318 | Yuan2021An | 0.26 | 0.00 | 0.00 | 0.00 | 0.00 | 0.00 | 0.00 | 0.00 | 0.00 | 0.74 |
| 319 | Zhang2021A | 0.00 | 0.00 | 0.00 | 0.63 | 0.00 | 0.24 | 0.00 | 0.00 | 0.00 | 0.13 |
| 320 | Zhang2021MI3 | 0.00 | 0.00 | 0.26 | 0.00 | 0.01 | 0.03 | 0.04 | 0.65 | 0.00 | 0.00 |
| 321 | Zhou2021Facilitating | 0.24 | 0.04 | 0.00 | 0.58 | 0.00 | 0.00 | 0.00 | 0.00 | 0.00 | 0.14 |
| 322 | Zytek2021Sibyl | 1.00 | 0.00 | 0.00 | 0.00 | 0.00 | 0.00 | 0.00 | 0.00 | 0.00 | 0.00 |
| 323 | Ahmed2022AutoCl | 0.00 | 0.00 | 0.00 | 0.00 | 0.43 | 0.00 | 0.00 | 0.00 | 0.00 | 0.57 |
| 324 | Antweiler2022Visualizing | 0.00 | 0.16 | 0.00 | 0.00 | 0.00 | 0.00 | 0.00 | 0.00 | 0.00 | 0.84 |
| 325 | Appleby2022HyperNP | 0.00 | 0.00 | 0.00 | 0.00 | 1.00 | 0.00 | 0.00 | 0.00 | 0.00 | 0.00 |
| 326 | Balayn2022How | 0.90 | 0.00 | 0.00 | 0.00 | 0.09 | 0.00 | 0.00 | 0.01 | 0.00 | 0.00 |
| 327 | Bauerle2022exploRNN | 0.18 | 0.00 | 0.74 | 0.00 | 0.00 | 0.00 | 0.00 | 0.00 | 0.00 | 0.08 |
| 328 | Bauerle2022Symphony | 0.00 | 0.00 | 0.00 | 0.00 | 0.00 | 0.00 | 0.00 | 0.04 | 0.00 | 0.96 |
| 329 | Beckmann2022Interactive | 0.00 | 0.00 | 0.00 | 0.00 | 0.18 | 0.00 | 0.00 | 0.82 | 0.00 | 0.00 |
| 330 | Bodria2022Explaining | 0.05 | 0.14 | 0.00 | 0.06 | 0.58 | 0.00 | 0.00 | 0.00 | 0.17 | 0.00 |

Table 6: The topic modeling results for our survey (continued).

| # | Technique | Topic_1 | Topic_2 | Topic_3 | Topic_4 | Topic_5 | Topic_6 | Topic_7 | Topic_8 | Topic_9 | Topic_10 |
|---|---|---|---|---|---|---|---|---|---|---|---|
| 331 | Boggust2022Embedding | 0.00 | 0.00 | 0.00 | 0.26 | 0.00 | 0.00 | 0.00 | 0.74 | 0.00 | 0.00 |
| 332 | Boggust2022Shared | 0.00 | 0.00 | 0.00 | 0.00 | 0.00 | 0.00 | 0.00 | 1.00 | 0.00 | 0.00 |
| 333 | Bredius2022Visual | 0.00 | 0.00 | 0.00 | 0.00 | 1.00 | 0.00 | 0.00 | 0.00 | 0.00 | 0.00 |
| 334 | Chatzimparmpas2022FeatureEnVi | 0.00 | 0.34 | 0.00 | 0.00 | 0.30 | 0.02 | 0.00 | 0.00 | 0.11 | 0.23 |
| 335 | Chen2022HINT | 0.33 | 0.00 | 0.00 | 0.00 | 0.00 | 0.00 | 0.00 | 0.00 | 0.00 | 0.67 |
| 336 | Chen2022Towards | 0.00 | 0.00 | 0.36 | 0.00 | 0.00 | 0.46 | 0.00 | 0.00 | 0.18 | 0.00 |
| 337 | Cheng2022A | 0.00 | 0.73 | 0.11 | 0.00 | 0.00 | 0.00 | 0.00 | 0.00 | 0.04 | 0.13 |
| 338 | Cheng2022ACMViz | 0.00 | 0.00 | 1.00 | 0.00 | 0.00 | 0.00 | 0.00 | 0.00 | 0.00 | 0.00 |
| 339 | Cheng2022VBridge | 0.45 | 0.00 | 0.25 | 0.00 | 0.00 | 0.00 | 0.00 | 0.00 | 0.14 | 0.16 |
| 340 | Cherepanov2022Visualization | 0.02 | 0.00 | 0.80 | 0.00 | 0.15 | 0.00 | 0.00 | 0.00 | 0.00 | 0.03 |
| 341 | Collaris2022Comparative | 0.40 | 0.00 | 0.00 | 0.00 | 0.40 | 0.00 | 0.14 | 0.00 | 0.00 | 0.06 |
| 342 | Collaris2022StrategyAtlas | 0.16 | 0.10 | 0.06 | 0.00 | 0.17 | 0.25 | 0.10 | 0.00 | 0.06 | 0.10 |
| 343 | Eckelt2022Visual | 0.00 | 0.02 | 0.00 | 0.14 | 0.00 | 0.84 | 0.00 | 0.00 | 0.00 | 0.00 |
| 344 | Eirich2022IRVINE | 0.00 | 0.00 | 0.00 | 0.00 | 0.00 | 0.11 | 0.22 | 0.18 | 0.41 | 0.08 |
| 345 | Eirich2022RfX | 0.00 | 0.28 | 0.00 | 0.00 | 0.02 | 0.34 | 0.00 | 0.00 | 0.06 | 0.29 |
| 346 | Fujiwara2022Interactive | 0.00 | 0.04 | 0.00 | 0.78 | 0.00 | 0.05 | 0.14 | 0.00 | 0.00 | 0.00 |
| 347 | Gobbo2022xai | 0.17 | 0.00 | 0.10 | 0.00 | 0.00 | 0.20 | 0.00 | 0.02 | 0.00 | 0.51 |
| 348 | Gortler2022Neo | 0.00 | 0.00 | 0.00 | 0.00 | 0.15 | 0.63 | 0.00 | 0.06 | 0.00 | 0.15 |
| 349 | Grimmeisen2022VisGIL | 0.00 | 0.00 | 0.00 | 0.00 | 0.00 | 0.03 | 0.02 | 0.94 | 0.00 | 0.00 |
| 350 | Haedecke2022ScrutinAI | 0.05 | 0.00 | 0.38 | 0.00 | 0.00 | 0.00 | 0.50 | 0.00 | 0.00 | 0.07 |
| 351 | Han2022Explainable | 0.04 | 0.00 | 0.05 | 0.00 | 0.51 | 0.41 | 0.00 | 0.00 | 0.00 | 0.00 |
| 352 | He2022Where | 0.00 | 0.03 | 0.95 | 0.00 | 0.00 | 0.00 | 0.00 | 0.00 | 0.02 | 0.00 |
| 353 | Hinterreiter2022ConfusionFlow | 0.00 | 0.00 | 0.02 | 0.00 | 0.83 | 0.00 | 0.01 | 0.15 | 0.00 | 0.00 |
| 354 | Hografer2022Steering | 0.08 | 0.06 | 0.00 | 0.00 | 0.23 | 0.00 | 0.53 | 0.10 | 0.00 | 0.00 |
| 355 | Horak2022Visual | 0.01 | 0.00 | 0.03 | 0.00 | 0.00 | 0.00 | 0.00 | 0.95 | 0.00 | 0.00 |
| 356 | Jeon2022Measuring | 0.00 | 0.00 | 0.00 | 0.29 | 0.02 | 0.05 | 0.64 | 0.00 | 0.00 | 0.00 |
| 357 | Jeong2022Interactively | 0.00 | 0.60 | 0.02 | 0.00 | 0.36 | 0.00 | 0.00 | 0.00 | 0.00 | 0.00 |
| 358 | Jin2022GNNLens | 0.00 | 0.00 | 0.00 | 0.00 | 0.03 | 0.00 | 0.00 | 0.00 | 0.97 | 0.00 |
| 359 | Kaul2022Improving | 0.94 | 0.06 | 0.00 | 0.00 | 0.00 | 0.00 | 0.00 | 0.00 | 0.00 | 0.00 |
| 360 | Knittel2022Real | 0.00 | 0.00 | 0.00 | 0.00 | 0.00 | 0.92 | 0.02 | 0.00 | 0.06 | 0.00 |
| 361 | Konforti2022SIGN | 0.00 | 0.00 | 0.34 | 0.00 | 0.20 | 0.00 | 0.37 | 0.00 | 0.07 | 0.00 |
| 362 | Kwon2022DASH | 0.24 | 0.00 | 0.04 | 0.00 | 0.69 | 0.03 | 0.00 | 0.00 | 0.00 | 0.00 |
| 363 | Kwon2022RMExplorer | 0.37 | 0.06 | 0.00 | 0.00 | 0.00 | 0.00 | 0.00 | 0.00 | 0.00 | 0.58 |
| 364 | Li2022A | 0.01 | 0.00 | 0.11 | 0.11 | 0.05 | 0.00 | 0.00 | 0.00 | 0.72 | 0.00 |
| 365 | Liu2022Visualizing | 0.00 | 0.00 | 0.00 | 0.05 | 0.14 | 0.00 | 0.00 | 0.01 | 0.79 | 0.00 |
| 366 | Loreaux2022Boosting | 0.45 | 0.00 | 0.06 | 0.00 | 0.00 | 0.00 | 0.00 | 0.00 | 0.05 | 0.44 |
| 367 | Marcilio2022Semi | 0.00 | 0.00 | 0.23 | 0.00 | 0.68 | 0.04 | 0.05 | 0.00 | 0.00 | 0.00 |
| 368 | Medoc2022Visualizing | 0.08 | 0.46 | 0.00 | 0.00 | 0.23 | 0.00 | 0.00 | 0.06 | 0.00 | 0.18 |
| 369 | Meng2022ModelWise | 0.13 | 0.02 | 0.00 | 0.00 | 0.82 | 0.00 | 0.00 | 0.00 | 0.03 | 0.00 |
| 370 | Metz2022A | 0.00 | 0.00 | 0.72 | 0.00 | 0.00 | 0.00 | 0.00 | 0.06 | 0.00 | 0.21 |
| 371 | Mishra2022Why | 0.27 | 0.01 | 0.51 | 0.00 | 0.00 | 0.00 | 0.00 | 0.21 | 0.00 | 0.00 |
| 372 | Monadjemi2022Guided | 0.14 | 0.00 | 0.00 | 0.00 | 0.00 | 0.28 | 0.00 | 0.37 | 0.00 | 0.20 |
| 373 | Munechika2022Visual | 0.13 | 0.00 | 0.00 | 0.00 | 0.00 | 0.00 | 0.00 | 0.00 | 0.00 | 0.87 |
| 374 | Munz2022Visualization | 0.00 | 0.00 | 0.00 | 1.00 | 0.00 | 0.00 | 0.00 | 0.00 | 0.00 | 0.00 |
| 375 | Nakao2022Toward | 1.00 | 0.00 | 0.00 | 0.00 | 0.00 | 0.00 | 0.00 | 0.00 | 0.00 | 0.00 |
| 376 | Neto2022Multivariate | 0.00 | 0.42 | 0.00 | 0.00 | 0.06 | 0.02 | 0.00 | 0.50 | 0.00 | 0.00 |
| 377 | Neves2022Fast | 0.00 | 0.00 | 0.00 | 0.00 | 0.35 | 0.40 | 0.24 | 0.00 | 0.00 | 0.00 |
| 378 | Nourani2022DETOXER | 0.61 | 0.00 | 0.02 | 0.00 | 0.04 | 0.00 | 0.00 | 0.01 | 0.24 | 0.09 |
| 379 | Oliveira2022SDBM | 0.00 | 0.00 | 0.00 | 0.00 | 1.00 | 0.00 | 0.00 | 0.00 | 0.00 | 0.00 |
| 380 | Palmeiro2022Data | 0.00 | 0.00 | 0.15 | 0.00 | 0.01 | 0.00 | 0.31 | 0.00 | 0.08 | 0.45 |
| 381 | Park2022NeuroCartography | 0.00 | 0.00 | 0.00 | 0.01 | 0.94 | 0.04 | 0.00 | 0.00 | 0.00 | 0.00 |
| 382 | Pu2022matExplorer | 0.00 | 0.06 | 0.00 | 0.00 | 0.00 | 0.00 | 0.00 | 0.00 | 0.94 | 0.00 |
| 383 | Qian2022RCDVis | 0.00 | 0.00 | 0.00 | 0.00 | 0.00 | 0.00 | 0.00 | 0.00 | 1.00 | 0.00 |
| 384 | Ratzenbock2022Uncover | 0.00 | 0.00 | 0.00 | 0.00 | 0.00 | 0.67 | 0.00 | 0.00 | 0.33 | 0.00 |
| 385 | Rind2022Trustworthy | 0.70 | 0.00 | 0.10 | 0.00 | 0.13 | 0.00 | 0.04 | 0.00 | 0.03 | 0.00 |
| 386 | Rostamzadeh2022Visual | 0.00 | 0.11 | 0.00 | 0.00 | 0.00 | 0.00 | 0.00 | 0.09 | 0.00 | 0.80 |
| 387 | Schafer2022Interactive | 0.19 | 0.07 | 0.15 | 0.12 | 0.00 | 0.00 | 0.00 | 0.00 | 0.00 | 0.46 |
| 388 | Schlegel2022ViNNPruner | 0.00 | 0.00 | 0.34 | 0.00 | 0.24 | 0.00 | 0.42 | 0.00 | 0.00 | 0.00 |
| 389 | Sevastjanova2022LMFingerprints | 0.00 | 0.00 | 0.19 | 0.63 | 0.00 | 0.00 | 0.00 | 0.18 | 0.00 | 0.00 |
| 390 | Shrestha2022FairFuse | 0.48 | 0.08 | 0.00 | 0.00 | 0.00 | 0.00 | 0.00 | 0.00 | 0.14 | 0.30 |
| 391 | Sielaff2022Visual | 0.08 | 0.08 | 0.00 | 0.00 | 0.00 | 0.00 | 0.00 | 0.00 | 0.35 | 0.49 |
| 392 | Sivaraman2022Emblaze | 0.06 | 0.00 | 0.00 | 0.56 | 0.02 | 0.04 | 0.00 | 0.27 | 0.00 | 0.05 |
| 393 | Sohns2022Attribute | 0.00 | 0.24 | 0.00 | 0.14 | 0.46 | 0.00 | 0.11 | 0.00 | 0.00 | 0.06 |
| 394 | Strobelt2022GenNI | 0.00 | 0.63 | 0.06 | 0.00 | 0.00 | 0.00 | 0.00 | 0.09 | 0.16 | 0.07 |
| 395 | Suresh2022Intuitively | 0.53 | 0.00 | 0.00 | 0.00 | 0.12 | 0.00 | 0.00 | 0.35 | 0.00 | 0.00 |
| 396 | Theissler2022ConfusionVis | 0.01 | 0.00 | 0.00 | 0.00 | 0.99 | 0.00 | 0.00 | 0.00 | 0.00 | 0.00 |
| 397 | Varu2022ARMatrix | 0.00 | 0.04 | 0.00 | 0.00 | 0.00 | 0.22 | 0.00 | 0.00 | 0.00 | 0.74 |
| 398 | Velumani2022AQX | 0.07 | 0.00 | 0.86 | 0.00 | 0.00 | 0.00 | 0.00 | 0.00 | 0.07 | 0.00 |
| 399 | Wang2022Interpretability | 0.02 | 0.00 | 0.00 | 0.00 | 0.00 | 0.00 | 0.00 | 0.00 | 0.00 | 0.98 |
| 400 | Wang2022Learning | 0.00 | 0.04 | 0.07 | 0.00 | 0.64 | 0.00 | 0.00 | 0.00 | 0.21 | 0.04 |

Table 7: The topic modeling results for our survey (continued).

| # | **Technique** | Topic_1 | Topic_2 | Topic_3 | Topic_4 | Topic_5 | Topic_6 | Topic_7 | Topic_8 | Topic_9 | Topic_10 |
|---|---|---|---|---|---|---|---|---|---|---|---|
| 401 | Wang2022M2Lens | 0.05 | 0.00 | 0.00 | 0.10 | 0.00 | 0.00 | 0.00 | 0.11 | 0.74 | 0.00 |
| 402 | Wang2022TimberTrek | 0.00 | 0.44 | 0.02 | 0.00 | 0.00 | 0.00 | 0.00 | 0.00 | 0.00 | 0.54 |
| 403 | Wang2022When | 0.00 | 0.00 | 0.95 | 0.00 | 0.00 | 0.00 | 0.00 | 0.00 | 0.05 | 0.00 |
| 404 | Witschard2022Interactive | 0.00 | 0.00 | 0.00 | 0.15 | 0.00 | 0.52 | 0.00 | 0.32 | 0.00 | 0.01 |
| 405 | Worland2022Visualization | 0.00 | 1.00 | 0.00 | 0.00 | 0.00 | 0.00 | 0.00 | 0.00 | 0.00 | 0.00 |
| 406 | Xie2022FairRankVis | 0.23 | 0.00 | 0.00 | 0.00 | 0.00 | 0.00 | 0.00 | 0.00 | 0.77 | 0.00 |
| 407 | Xuan2022VAC | 0.34 | 0.00 | 0.16 | 0.00 | 0.50 | 0.00 | 0.00 | 0.00 | 0.00 | 0.00 |
| 408 | Yang2022Diagnosing | 0.00 | 0.00 | 0.01 | 0.54 | 0.19 | 0.08 | 0.00 | 0.03 | 0.14 | 0.00 |
| 409 | Yuan2022Context | 0.32 | 0.00 | 0.01 | 0.00 | 0.07 | 0.00 | 0.00 | 0.24 | 0.03 | 0.33 |
| 410 | Yuan2022iSEA | 0.04 | 0.00 | 0.00 | 0.13 | 0.00 | 0.00 | 0.00 | 0.19 | 0.00 | 0.64 |
| 411 | Yuan2022SUBPLEX | 0.28 | 0.00 | 0.00 | 0.00 | 0.00 | 0.07 | 0.00 | 0.00 | 0.47 | 0.16 |
| 412 | Yuan2022VisualExploration | 0.00 | 0.15 | 0.00 | 0.00 | 0.00 | 0.00 | 0.00 | 0.05 | 0.00 | 0.80 |
| 413 | Zang2022EVNet | 0.08 | 0.00 | 0.01 | 0.00 | 0.50 | 0.21 | 0.07 | 0.00 | 0.13 | 0.00 |
| 414 | Zhang2022HyIDSVis | 0.00 | 0.00 | 0.00 | 0.00 | 0.03 | 0.00 | 0.00 | 0.00 | 0.78 | 0.19 |
| 415 | Zhang2022OneLabeler | 0.00 | 0.00 | 0.00 | 0.00 | 0.00 | 0.00 | 0.00 | 0.98 | 0.00 | 0.02 |
| 416 | Zhao2022Human | 0.00 | 0.00 | 0.19 | 0.00 | 0.60 | 0.00 | 0.00 | 0.21 | 0.00 | 0.00 |
| 417 | Zhou2022NeuroMapper | 0.00 | 0.00 | 0.33 | 0.13 | 0.54 | 0.00 | 0.00 | 0.00 | 0.00 | 0.00 |
| 418 | Zytek2022Sibyl | 0.82 | 0.00 | 0.00 | 0.00 | 0.00 | 0.00 | 0.00 | 0.00 | 0.17 | 0.01 |
| 419 | Adilova2023Re | 0.00 | 0.11 | 0.00 | 0.00 | 0.18 | 0.00 | 0.03 | 0.00 | 0.00 | 0.68 |
| 420 | Ahn2023ESCAPE | 0.17 | 0.00 | 0.00 | 0.00 | 0.60 | 0.00 | 0.00 | 0.23 | 0.00 | 0.00 |
| 421 | Alexandre2023Visual | 0.45 | 0.15 | 0.00 | 0.14 | 0.00 | 0.00 | 0.00 | 0.27 | 0.00 | 0.00 |
| 422 | Angelini2023A | 0.07 | 0.00 | 0.00 | 0.00 | 0.00 | 0.00 | 0.75 | 0.00 | 0.18 | 0.00 |
| 423 | Arnorsson2023Why | 0.10 | 0.00 | 0.00 | 0.00 | 0.00 | 0.10 | 0.00 | 0.14 | 0.00 | 0.66 |
| 424 | Arunkumar2023LINGO | 0.00 | 0.00 | 0.00 | 0.00 | 0.00 | 0.00 | 0.00 | 1.00 | 0.00 | 0.00 |
| 425 | Atzberger2023Large | 0.00 | 0.56 | 0.00 | 0.10 | 0.00 | 0.28 | 0.00 | 0.00 | 0.00 | 0.06 |
| 426 | Babu2023User | 0.09 | 0.00 | 0.00 | 0.00 | 0.00 | 0.00 | 0.00 | 0.00 | 0.00 | 0.91 |
| 427 | Bertucci2023DendroMap | 0.04 | 0.00 | 0.00 | 0.00 | 0.40 | 0.50 | 0.00 | 0.00 | 0.00 | 0.06 |
| 428 | Bienefeld2023Solving | 0.72 | 0.00 | 0.00 | 0.00 | 0.00 | 0.00 | 0.00 | 0.00 | 0.00 | 0.28 |
| 429 | Bykov2023DORA | 0.00 | 0.00 | 0.16 | 0.00 | 0.83 | 0.00 | 0.00 | 0.00 | 0.00 | 0.00 |
| 430 | Cabral2023Addressing | 0.00 | 0.00 | 0.00 | 0.17 | 0.00 | 0.71 | 0.00 | 0.07 | 0.00 | 0.05 |
| 431 | Cabrera2023Zeno | 0.00 | 0.00 | 0.00 | 0.00 | 0.00 | 0.00 | 0.00 | 0.04 | 0.00 | 0.96 |
| 432 | Chatzimparmpas2023HardVis | 0.00 | 0.00 | 0.00 | 0.00 | 0.67 | 0.06 | 0.00 | 0.05 | 0.07 | 0.15 |
| 433 | Chatzimparmpas2023VisRuler | 0.06 | 0.27 | 0.00 | 0.00 | 0.14 | 0.04 | 0.00 | 0.23 | 0.00 | 0.25 |
| 434 | Chen2023A | 0.09 | 0.09 | 0.59 | 0.00 | 0.17 | 0.00 | 0.00 | 0.00 | 0.06 | 0.00 |
| 435 | Chen2023Federated | 0.02 | 0.03 | 0.69 | 0.00 | 0.00 | 0.11 | 0.00 | 0.00 | 0.08 | 0.08 |
| 436 | Cheng2023Polyphony | 0.00 | 0.00 | 0.00 | 0.00 | 0.00 | 0.11 | 0.00 | 0.00 | 0.87 | 0.03 |
| 437 | Chu2023A | 0.00 | 0.02 | 0.00 | 0.00 | 0.17 | 0.00 | 0.04 | 0.00 | 0.53 | 0.25 |
| 438 | Collaris2023LEMON | 0.04 | 0.00 | 0.00 | 0.00 | 0.96 | 0.00 | 0.00 | 0.00 | 0.00 | 0.00 |
| 439 | Delaforge2023EBBE | 0.02 | 0.81 | 0.00 | 0.10 | 0.02 | 0.00 | 0.00 | 0.03 | 0.02 | 0.00 |
| 440 | Deng2023Visual | 0.00 | 0.00 | 0.00 | 0.68 | 0.00 | 0.00 | 0.00 | 0.12 | 0.20 | 0.00 |
| 441 | Dilawer2023MultiCaM | 0.11 | 0.42 | 0.04 | 0.00 | 0.43 | 0.00 | 0.00 | 0.00 | 0.00 | 0.00 |
| 442 | Feng2023PromptMagician | 0.00 | 0.00 | 0.12 | 0.00 | 0.00 | 0.46 | 0.00 | 0.42 | 0.00 | 0.00 |
| 443 | Feng2023XNLI | 0.89 | 0.00 | 0.00 | 0.00 | 0.00 | 0.00 | 0.00 | 0.00 | 0.10 | 0.00 |
| 444 | Floricel2023Roses | 0.40 | 0.00 | 0.00 | 0.26 | 0.00 | 0.09 | 0.00 | 0.00 | 0.00 | 0.25 |
| 445 | Fujiwara2023Feature | 0.00 | 0.09 | 0.00 | 0.70 | 0.03 | 0.17 | 0.00 | 0.00 | 0.00 | 0.00 |
| 446 | Ge2023Optimally | 0.00 | 0.42 | 0.00 | 0.00 | 0.00 | 0.31 | 0.00 | 0.00 | 0.27 | 0.00 |
| 447 | Ghai2023D | 0.77 | 0.11 | 0.00 | 0.06 | 0.00 | 0.00 | 0.01 | 0.00 | 0.03 | 0.02 |
| 448 | Guo2023Causalvis | 0.37 | 0.00 | 0.00 | 0.00 | 0.00 | 0.00 | 0.00 | 0.00 | 0.00 | 0.63 |
| 449 | Haedecke2023ScrutinAI | 0.06 | 0.00 | 0.42 | 0.00 | 0.02 | 0.00 | 0.45 | 0.00 | 0.00 | 0.04 |
| 450 | Hao2023TimeTuner | 0.11 | 0.26 | 0.00 | 0.00 | 0.00 | 0.00 | 0.00 | 0.00 | 0.63 | 0.00 |
| 451 | He2023VideoPro | 0.00 | 0.00 | 0.03 | 0.00 | 0.00 | 0.00 | 0.00 | 0.49 | 0.48 | 0.00 |
| 452 | Hilasaca2023A | 0.00 | 0.62 | 0.00 | 0.00 | 0.09 | 0.01 | 0.12 | 0.00 | 0.16 | 0.00 |
| 453 | Hografer2023Tailorable | 0.00 | 0.00 | 0.00 | 0.00 | 0.00 | 0.00 | 1.00 | 0.00 | 0.00 | 0.00 |
| 454 | Hong2023Visualizing | 0.12 | 0.00 | 0.00 | 0.00 | 0.00 | 0.00 | 0.00 | 0.00 | 0.74 | 0.13 |
| 455 | Hoque2023Visual | 0.00 | 0.00 | 0.29 | 0.00 | 0.00 | 0.00 | 0.00 | 0.61 | 0.09 | 0.00 |
| 456 | Horak2023xOpat | 0.00 | 0.00 | 0.23 | 0.00 | 0.09 | 0.00 | 0.03 | 0.00 | 0.00 | 0.65 |
| 457 | Hu2023Xaitk | 0.08 | 0.00 | 0.49 | 0.00 | 0.11 | 0.00 | 0.00 | 0.16 | 0.00 | 0.17 |
| 458 | Huang2023A | 0.00 | 0.06 | 0.00 | 0.00 | 0.00 | 0.32 | 0.17 | 0.08 | 0.37 | 0.00 |
| 459 | Huang2023ConceptExplainer | 0.05 | 0.00 | 0.02 | 0.00 | 0.27 | 0.00 | 0.00 | 0.66 | 0.00 | 0.00 |
| 460 | Jeon2023CLAMS | 0.08 | 0.00 | 0.00 | 0.00 | 0.00 | 0.17 | 0.75 | 0.00 | 0.00 | 0.00 |
| 461 | Jeon2023Classes | 0.00 | 0.00 | 0.00 | 0.51 | 0.14 | 0.16 | 0.11 | 0.08 | 0.00 | 0.00 |
| 462 | Jeon2023ZADU | 0.00 | 0.00 | 0.00 | 0.93 | 0.00 | 0.00 | 0.05 | 0.00 | 0.00 | 0.02 |
| 463 | Jeong2023Dimensionality | 0.00 | 0.00 | 0.00 | 0.00 | 0.00 | 0.22 | 0.00 | 0.00 | 0.78 | 0.00 |
| 464 | Jin2023A | 0.00 | 0.00 | 0.09 | 0.14 | 0.00 | 0.00 | 0.00 | 0.00 | 0.77 | 0.00 |
| 465 | Jin2023ShortcutLens | 0.00 | 0.00 | 0.00 | 0.00 | 0.00 | 0.00 | 0.00 | 0.05 | 0.95 | 0.00 |
| 466 | Joo2023Distributional | 0.20 | 0.00 | 0.00 | 0.00 | 0.33 | 0.00 | 0.46 | 0.00 | 0.00 | 0.00 |
| 467 | Kadir2023A | 0.48 | 0.00 | 0.29 | 0.00 | 0.13 | 0.00 | 0.00 | 0.11 | 0.00 | 0.00 |
| 468 | Kale2023EVM | 0.64 | 0.02 | 0.00 | 0.00 | 0.00 | 0.00 | 0.10 | 0.00 | 0.04 | 0.19 |
| 469 | Kerrigan2023SliceLens | 0.00 | 0.16 | 0.00 | 0.00 | 0.00 | 0.00 | 0.00 | 0.15 | 0.00 | 0.68 |
| 470 | Klaus2023A | 0.00 | 0.80 | 0.00 | 0.00 | 0.00 | 0.00 | 0.00 | 0.00 | 0.00 | 0.20 |

Table 8: The topic modeling results for our survey (concluded).

| # | Technique | Topic_1 | Topic_2 | Topic_3 | Topic_4 | Topic_5 | Topic_6 | Topic_7 | Topic_8 | Topic_9 | Topic_10 |
|---|---|---|---|---|---|---|---|---|---|---|---|
| 471 | Kwon2023Finspector | 0.16 | 0.02 | 0.00 | 0.47 | 0.00 | 0.00 | 0.00 | 0.09 | 0.07 | 0.18 |
| 472 | Lan2023MediVizor | 0.71 | 0.00 | 0.00 | 0.00 | 0.00 | 0.00 | 0.00 | 0.00 | 0.29 | 0.00 |
| 473 | Li2023How | 0.00 | 0.00 | 0.08 | 0.92 | 0.00 | 0.00 | 0.00 | 0.00 | 0.00 | 0.00 |
| 474 | Li2023Incorporation | 0.01 | 0.23 | 0.00 | 0.00 | 0.11 | 0.62 | 0.00 | 0.02 | 0.00 | 0.00 |
| 475 | Li2023ScatterUQ | 0.02 | 0.00 | 0.03 | 0.00 | 0.88 | 0.00 | 0.01 | 0.02 | 0.00 | 0.03 |
| 476 | Li2023SpectrumVA | 0.00 | 0.00 | 0.33 | 0.00 | 0.02 | 0.00 | 0.00 | 0.00 | 0.64 | 0.00 |
| 477 | Li2023Visual | 0.00 | 0.00 | 0.18 | 0.00 | 0.21 | 0.00 | 0.29 | 0.31 | 0.00 | 0.00 |
| 478 | Li2023VisualNeuron | 0.00 | 0.00 | 0.06 | 0.00 | 0.94 | 0.00 | 0.00 | 0.00 | 0.00 | 0.00 |
| 479 | Liu2023RankAxis | 0.03 | 0.31 | 0.00 | 0.00 | 0.07 | 0.03 | 0.24 | 0.00 | 0.20 | 0.12 |
| 480 | Lu2023Visual | 0.00 | 0.90 | 0.00 | 0.08 | 0.02 | 0.00 | 0.00 | 0.00 | 0.00 | 0.00 |
| 481 | Machado2023ShaRP | 0.00 | 0.00 | 0.00 | 0.00 | 0.77 | 0.23 | 0.00 | 0.00 | 0.00 | 0.00 |
| 482 | Meng2023Class | 0.00 | 0.00 | 0.00 | 0.00 | 0.78 | 0.16 | 0.00 | 0.06 | 0.00 | 0.00 |
| 483 | Metz2023VISITOR | 0.00 | 0.00 | 0.65 | 0.02 | 0.00 | 0.03 | 0.00 | 0.30 | 0.00 | 0.00 |
| 484 | Mir2023Circles | 0.00 | 0.15 | 0.00 | 0.00 | 0.68 | 0.00 | 0.00 | 0.00 | 0.00 | 0.16 |
| 485 | Mobaraki2023A | 0.01 | 0.00 | 0.09 | 0.00 | 0.28 | 0.00 | 0.00 | 0.16 | 0.33 | 0.12 |
| 486 | Morariu2023DumbleDR | 0.04 | 0.02 | 0.00 | 0.00 | 0.68 | 0.16 | 0.00 | 0.00 | 0.00 | 0.10 |
| 487 | Morgenshtern2023RiskFix | 0.05 | 0.00 | 0.00 | 0.00 | 0.00 | 0.00 | 0.00 | 0.00 | 0.00 | 0.95 |
| 488 | Onzenoodt2023Out | 0.02 | 0.00 | 0.00 | 0.00 | 0.00 | 0.98 | 0.00 | 0.00 | 0.00 | 0.00 |
| 489 | Piccolotto2023Data | 0.07 | 0.00 | 0.00 | 0.00 | 0.44 | 0.21 | 0.29 | 0.00 | 0.00 | 0.00 |
| 490 | Ploshchik2023MetaStackVis | 0.00 | 0.00 | 0.00 | 0.00 | 0.18 | 0.44 | 0.00 | 0.00 | 0.00 | 0.38 |
| 491 | Pomme2023NetPrune | 0.00 | 0.00 | 0.03 | 0.00 | 0.70 | 0.00 | 0.26 | 0.00 | 0.00 | 0.00 |
| 492 | Prasad2023ProactiV | 0.00 | 0.00 | 0.00 | 0.00 | 1.00 | 0.00 | 0.00 | 0.00 | 0.00 | 0.00 |
| 493 | Prasad2023The | 0.00 | 0.00 | 0.03 | 0.00 | 0.87 | 0.00 | 0.00 | 0.04 | 0.00 | 0.06 |
| 494 | Quadri2023Automatic | 0.00 | 0.00 | 0.00 | 0.00 | 0.05 | 0.75 | 0.19 | 0.00 | 0.00 | 0.00 |
| 495 | Ramsey2023Toward | 0.18 | 0.29 | 0.00 | 0.00 | 0.00 | 0.00 | 0.00 | 0.27 | 0.00 | 0.26 |
| 496 | Rathore2023VERB | 0.07 | 0.00 | 0.00 | 0.38 | 0.00 | 0.10 | 0.00 | 0.45 | 0.00 | 0.00 |
| 497 | Reif2023Visualizing | 0.00 | 0.00 | 0.00 | 0.37 | 0.00 | 0.21 | 0.00 | 0.26 | 0.00 | 0.16 |
| 498 | Robertson2023Angler | 0.00 | 0.00 | 0.00 | 0.15 | 0.00 | 0.00 | 0.00 | 0.00 | 0.00 | 0.85 |
| 499 | Schlegel2023Interactive | 0.00 | 0.00 | 0.00 | 0.00 | 0.22 | 0.16 | 0.62 | 0.00 | 0.00 | 0.00 |
| 500 | Sevastjanova2023Visual | 0.00 | 0.00 | 0.00 | 0.27 | 0.00 | 0.00 | 0.00 | 0.39 | 0.34 | 0.00 |
| 501 | Shao2023Visual | 0.01 | 0.04 | 0.10 | 0.12 | 0.00 | 0.00 | 0.00 | 0.07 | 0.65 | 0.00 |
| 502 | Shi2023MADDPGViz | 0.00 | 0.00 | 1.00 | 0.00 | 0.00 | 0.00 | 0.00 | 0.00 | 0.00 | 0.00 |
| 503 | Shi2023VDL | 0.00 | 0.00 | 0.00 | 0.00 | 1.00 | 0.00 | 0.00 | 0.00 | 0.00 | 0.00 |
| 504 | Shrestha2023Help | 0.73 | 0.00 | 0.00 | 0.00 | 0.00 | 0.00 | 0.00 | 0.00 | 0.00 | 0.27 |
| 505 | Simic2023XAIVIER | 0.35 | 0.00 | 0.05 | 0.00 | 0.01 | 0.00 | 0.00 | 0.00 | 0.00 | 0.59 |
| 506 | Sivaraman2023Ignore | 0.89 | 0.00 | 0.00 | 0.00 | 0.00 | 0.00 | 0.00 | 0.00 | 0.00 | 0.10 |
| 507 | Sohns2023Decision | 0.09 | 0.00 | 0.00 | 0.02 | 0.68 | 0.00 | 0.06 | 0.15 | 0.00 | 0.00 |
| 508 | Steinparz2023Visualizing | 0.00 | 0.00 | 0.00 | 0.00 | 0.52 | 0.00 | 0.11 | 0.00 | 0.00 | 0.38 |
| 509 | Strobelt2023Interactive | 0.00 | 0.00 | 0.00 | 0.00 | 0.00 | 0.00 | 0.00 | 0.94 | 0.00 | 0.06 |
| 510 | Sun2023Designing | 0.76 | 0.00 | 0.20 | 0.00 | 0.00 | 0.00 | 0.00 | 0.04 | 0.00 | 0.00 |
| 511 | Teng2023VISPUR | 0.66 | 0.02 | 0.00 | 0.09 | 0.00 | 0.00 | 0.00 | 0.00 | 0.00 | 0.23 |
| 512 | Thijssen2023Scaling | 0.20 | 0.00 | 0.00 | 0.00 | 0.63 | 0.17 | 0.00 | 0.00 | 0.00 | 0.00 |
| 513 | Troisemaine2023An | 0.72 | 0.09 | 0.00 | 0.00 | 0.00 | 0.00 | 0.00 | 0.00 | 0.00 | 0.18 |
| 514 | Tseng2023Collaborative | 0.33 | 0.00 | 0.11 | 0.00 | 0.02 | 0.00 | 0.00 | 0.00 | 0.00 | 0.54 |
| 515 | Tyagi2023NAS | 0.00 | 0.00 | 0.20 | 0.27 | 0.00 | 0.02 | 0.00 | 0.09 | 0.16 | 0.25 |
| 516 | Vieth2023ManiVault | 0.00 | 0.00 | 0.08 | 0.00 | 0.04 | 0.00 | 0.55 | 0.05 | 0.00 | 0.28 |
| 517 | Wang2023CommonsenseVIS | 0.00 | 0.00 | 0.00 | 0.02 | 0.00 | 0.00 | 0.00 | 0.82 | 0.16 | 0.00 |
| 518 | Wang2023DeepSeer | 0.17 | 0.00 | 0.10 | 0.00 | 0.00 | 0.00 | 0.00 | 0.65 | 0.08 | 0.00 |
| 519 | Wang2023DOMINO | 0.19 | 0.00 | 0.00 | 0.00 | 0.00 | 0.00 | 0.72 | 0.00 | 0.05 | 0.04 |
| 520 | Wang2023DRAVA | 0.02 | 0.00 | 0.12 | 0.00 | 0.00 | 0.82 | 0.00 | 0.04 | 0.00 | 0.00 |
| 521 | Wang2023Extending | 0.84 | 0.00 | 0.00 | 0.00 | 0.00 | 0.00 | 0.00 | 0.00 | 0.16 | 0.00 |
| 522 | Wang2023GAM | 0.02 | 0.00 | 0.00 | 0.00 | 0.00 | 0.00 | 0.00 | 0.00 | 0.00 | 0.98 |
| 523 | Wang2023HetVis | 0.00 | 0.00 | 0.39 | 0.00 | 0.14 | 0.46 | 0.00 | 0.00 | 0.00 | 0.00 |
| 524 | Wang2023Visual | 0.00 | 0.00 | 0.10 | 0.00 | 0.00 | 0.00 | 0.00 | 0.00 | 0.90 | 0.00 |
| 525 | Wang2023WebSHAP | 0.04 | 0.00 | 0.15 | 0.01 | 0.00 | 0.00 | 0.00 | 0.00 | 0.00 | 0.80 |
| 526 | Wang2023WizMap | 0.00 | 0.00 | 0.05 | 0.73 | 0.00 | 0.00 | 0.00 | 0.11 | 0.00 | 0.12 |
| 527 | Wentzel2023DASS | 0.27 | 0.00 | 0.00 | 0.02 | 0.00 | 0.31 | 0.00 | 0.00 | 0.00 | 0.41 |
| 528 | Wu2023ATICVis | 0.00 | 0.00 | 0.08 | 0.82 | 0.00 | 0.00 | 0.00 | 0.07 | 0.03 | 0.00 |
| 529 | Wu2023VizOPTICS | 0.00 | 0.00 | 0.00 | 0.00 | 0.00 | 1.00 | 0.00 | 0.00 | 0.00 | 0.00 |
| 530 | Xenopoulos2023Calibrate | 0.00 | 0.00 | 0.00 | 0.00 | 0.17 | 0.00 | 0.00 | 0.00 | 0.00 | 0.83 |
| 531 | Xenopoulos2023GALE | 0.22 | 0.00 | 0.00 | 0.36 | 0.42 | 0.00 | 0.00 | 0.00 | 0.00 | 0.00 |
| 532 | Xia2023Interactive | 0.00 | 0.00 | 0.00 | 0.06 | 0.09 | 0.68 | 0.00 | 0.00 | 0.17 | 0.00 |
| 533 | Xie2023Towards | 0.02 | 0.00 | 0.03 | 0.00 | 0.00 | 0.27 | 0.00 | 0.00 | 0.67 | 0.00 |
| 534 | Ye2023Visualizing | 0.00 | 0.01 | 0.04 | 0.00 | 0.14 | 0.00 | 0.00 | 0.00 | 0.00 | 0.80 |
| 535 | Yeh2023AttentionViz | 0.00 | 0.00 | 0.02 | 0.98 | 0.00 | 0.00 | 0.00 | 0.00 | 0.00 | 0.00 |
| 536 | Yen2023CrowdIDEA | 0.54 | 0.00 | 0.00 | 0.00 | 0.00 | 0.00 | 0.00 | 0.46 | 0.00 | 0.00 |
| 537 | Yuan2023Visual | 0.00 | 0.00 | 0.08 | 0.02 | 0.10 | 0.00 | 0.00 | 0.00 | 0.80 | 0.00 |
| 538 | Zeng2023iHELP | 0.00 | 0.00 | 0.00 | 0.92 | 0.08 | 0.00 | 0.00 | 0.00 | 0.00 | 0.00 |
| 539 | Zhang2023CohortVA | 0.00 | 0.00 | 0.00 | 0.00 | 0.00 | 0.00 | 0.00 | 0.06 | 0.36 | 0.58 |
| 540 | Zhang2023LabelVizier | 0.00 | 0.00 | 0.00 | 0.00 | 0.00 | 0.00 | 0.00 | 0.67 | 0.16 | 0.16 |
| 541 | Zhang2023SliceTeller | 0.00 | 0.00 | 0.11 | 0.00 | 0.24 | 0.00 | 0.00 | 0.00 | 0.00 | 0.65 |
| 542 | Zheng2023EmbeddingTree | 0.00 | 0.33 | 0.00 | 0.28 | 0.00 | 0.05 | 0.02 | 0.16 | 0.16 | 0.00 |
